# Supplementary material for: CAMEO: A Causal Transfer Learning Approach for Performance Optimization of Configurable Computer Systems
Source: arXiv:2306.07888 source file (2023-10-03)
Supplement: Supplementary file 1 [file appendix_backup.tex]

\appendix

\section{Appendix.}
\label{sec:appendix}
\subsection{Definitions and Background}
\noindent \textbf{Configuration Space $\mathcal{O}$. }
Let $\mathcal{O}_i$ indicate the $i^{th}$ configuration option of a system, which can be set to a range of different values (e.g., categorical, boolean, and numerical). The configuration space
is a Cartesian product of all options $\mathcal{O} = Dom(\mathcal{O}_1) \times ... \times Dom(\mathcal{O}_d$), where d is the number of options. A configuration $o$ is then a member of the configuration space $\mathcal{O}$ in which all options are set to a given value within the range of permitted values for that option.

\noindent \textbf{Environment Space $\mathcal{E}$.} We describe an environment $e$ drawn from a given environment space $\mathcal{E}$ which consists of possible combinations of hardware, workload, software and deployment topology. 

\noindent \textbf{Causal Performance Model $\mathcal{G}$.}
% ~\rayb{can we give a picture of CPM?}
A causal performance model (CPM), denoted by $\mathcal{G}$, is an acyclic directed mixed graph (ADMG) that provides the functional dependencies (e.g., how variations in one or multiple variables determine variations in other variables) between configuration options, system events, and performance objectives. While interpreting a CPM, we view the nodes as variables and the arrows as causal connections.

\noindent \textbf{Observation.}
In the \textit{observational} formulation, we measure the distribution of an outcome variable (e.g., \textsf{latency} $\mathcal{Y}$) given that we \textit{observe} another variable (e.g., \textsf{cpu frequency} $\mathcal{O}_{i}$ for $1 \leq i 
\leq d$) taking a certain value $o_i$ (e.g., $\mathcal{O}_{i}= o_i$), denoted by $Pr(\mathcal{Y}~|~\mathcal{O}_{i}= o_i)$. 
%This is a familiar expression that, given adequate data, modern supervised machine learning algorithms can estimate.

\noindent \textbf{Intervention.} The \textit{interventional} inference tackles a harder task of estimating the  effects of deliberate actions. For example, we measure how the distribution of an outcome (e.g., \textsf{latency} $\mathcal{Y}$) would change if we (artificially) intervened during the data gathering process by forcing the variable \textsf{cpu frequency} $\mathcal{O}_{i}$ to a certain value $o_i$, but otherwise retain the other variables (e.g., \textsf{dirty ratio}) as is. We can estimate the outcome of the artificial intervention by modifying the CPM to reflect our intervention and applying Pearl's \emph{do-calculus}~\cite{pearl2009causality} which is denoted by $Pr(\mathcal{Y}~|~do(\mathcal{O}_{i}= o_i))$. Unlike observations, there is a structural change of CPM due to intervention that goes along with a change of probability distribution over the variables.



\noindent \textbf{Bayesian Optimization.} 
Bayesian Optimization (BO) is an efficient framework to solve global optimization problems using black-box evaluations of expensive performance objectives $\mathcal{Y}$. A typical BO approach consists two main elements: the surrogate model and the acquisition function. The surrogate models are trained with a small number of configuration measurements and are used to predict the objective functions value $\hat{\mathcal{Y}} = f(o)$ using predictive mean $\mu(o)$ and uncertainty $\sigma(o)$ for configurations $o \in \mathcal{O}$. A common practice is to use Gaussian processes (GPs) as surrogate model where the GP distribution over $f(o)$ is fully specified by its mean function its mean function $\mu(o)$  and its covariance function $k_c(o,o')$. The kernel or covariance function $k_c$ captures the regularity in the form of the correlation of the marginal distributions $f(o)$ and $f(o')$. After the surrogate model outputs predictive mean and uncertainty for the unseen configurations, \ourapproach needs an acquisition function to select the best configuration to sample. A good acquisition function should balance the trade-offs between exploration and exploitation. 




\subsection{Additional Motivational Example}
\begin{figure}[ht]
\centering
\includegraphics[width=0.3\textwidth]{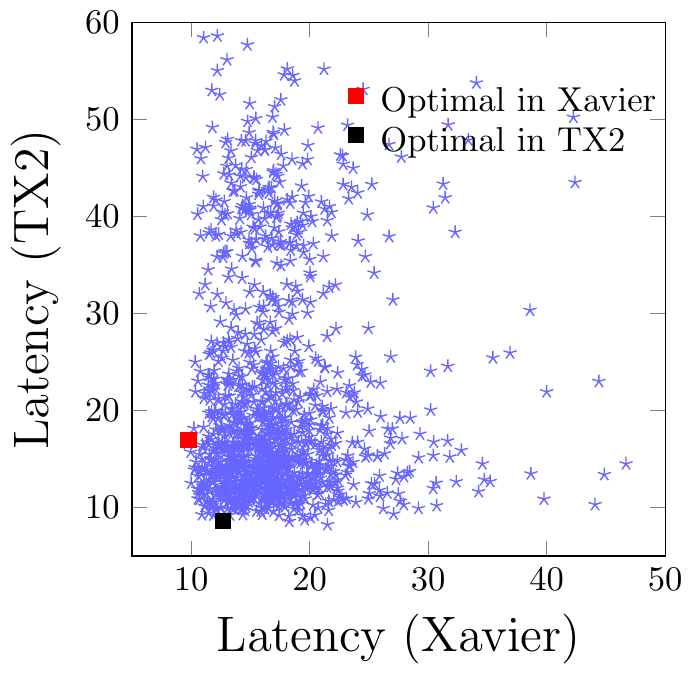}

\caption{\small{Optimal configuration for \textsc{MLPerf Object Detection} pipeline deployed on TX2 does not remain optimal on Xavier.
}}
    \label{fig:hw_change_intro}

\end{figure}
~\Cref{fig:hw_change_intro} shows a motivational example where the optimal configuration of an MLPerf Object Detection pipeline~\cite{reddi2020mlperf} on the Jetson TX2 device does not remain optimal on Jetson Xavier.



\subsection{Additional Details for Evaluation}
% \begin{figure*}[t!]
%     \centering
%     \resizebox{\linewidth}{!}{%
%     \begin{tabular}{ccccccc}
%     %  \clineB{2-5}{2.5}
%      \hline
%      \hline 
%      \multicolumn{1}{l}{\textsc{Method}}& \rotatebox{0}{\textsc{Search Strategy}} & \rotatebox{0}{\textsc{Category}} & \rotatebox{0}{\textsc{Reusable when distirbution shifts}} & \rotatebox{0}{\textsc{Type of Knowledge Reused}} & \rotatebox{0}{\textsc{Systems}} & \rotatebox{0}{\textsc{Configuration Space Size}} \\ 
%     %  \clineB{2-5}{2.5}
%      \hline 
     
%      %\multicolumn{1}{l}{} & \multicolumn{1}{l}{} & \multicolumn{1}{l}{}&
%      %\multicolumn{1}{l}{} &\multicolumn{1}{l}{} \\ \hline
     
%      \multicolumn{1}{l}{\textsc{SMAC}}~\cite{hutter2011sequential} & Sequential Model Based Optimization&Observation&Optimal within budget &No\\
     
    
     
%      \multicolumn{1}{l}{\textsc{Cello}}~\cite{ding2022cello} & Bayesian Optimization with Early Termination&Observation&Optimal under constraint on other objective&No\\
     
%      \multicolumn{1}{l}{\textsc{Cherrypick}}~\cite{alipourfard2017cherrypick} & Bayesian Optimization&Observation&Optimal within budget&No\\
     
%      \multicolumn{1}{l}{\textsc{Morphling}}~\cite{wang2021morphling} & Sequential Model Based Optimization and reuse with few shot&Observation&Optimal within budget&Yes\\
     
%      \multicolumn{1}{l}{\textsc{Scope}}~\cite{ding2021generalizable} & Observational Bayesian Optimization&Observation&Optimally Safe Configurations&Yes\\
     
%      \multicolumn{1}{l}{\textsc{OptimusCloud}}~\cite{mahgoub2020optimuscloud} & Dynamic Gradient Free Optimization&Observation&Optimal within budget&No\\
     
%      \multicolumn{1}{l}{\textsc{ResTune}}~\cite{zhang2021restune} & Observational Active Learning &Observation&Optimal within budget&Yes\\
%        \multicolumn{1}{l}{\textsc{Turbo}}~\cite{chen2021efficient} & Observational Active Learning  &Observation&Optimal within budget&Yes\\
%          \multicolumn{1}{l}{\textsc{Unicorn}}~\cite{iqbal2022unicorn} & Observational Active Learning with Causality &Observation&Optimal within budget&Yes\\
%       \multicolumn{1}{l}{\textsc{Jumbo}}~\cite{hakhamaneshi2021jumbo} & Obervation of features with maximum information & Observation& Optimal until Convergence&Yes\\
%      \hline 
%      \multicolumn{1}{l}{\ourapproach} & Counterfactual query estimation&Observation and Intervention&Optimal within budget&Yes\\
     
    
%     % \multicolumn{1}{V{2.5}l}{Search Strategy} & Gradient & Gradient & Gradient  & Scalarization &
%     %  Hypervolume & Maximum & Output Space &
%     %  Input Space  & Input Space & Chebyshev & Hypervolume of\\ 
     
%     %  \multicolumn{1}{V{2.5}l}{} & based & based & 
%     %   based&  &
%     %   improvement & Uncertainty & Entropy &
%     %  Entropy & Entropy& scalarization & Pareto region\\
%     %   \multicolumn{1}{V{2.5}l}{Evaluation Strategy} &  &  & 
%     %   & Coupled & Coupled &
%     %   Coupled& Coupled & Coupled &
%     %  Decoupled & Coupled & Decoupled\\
     
%     %  \multicolumn{1}{V{2.5}l}{Cost Awareness} &  $\cdot$ & $\cdot$&
%     %   &$\cdot$&$\cdot$&$\cdot$
%     %   &$\cdot$&$\cdot$&$\cdot$& \color{black}{\faCheck}& \color{black}{\faCheck} \\
      
%     %   \multicolumn{1}{V{2.5}l}{Tackles Stein's Paradox} &  $\cdot$ & $\cdot$&$\cdot$
%     %   &\color{black}{\faCheck}&\color{black}{\faCheck}&\color{black}{\faCheck}
%     %   &\color{black}{\faCheck}&\color{black}{\faCheck}&$\cdot$& \color{black}{\faCheck}& \color{black}{\faCheck} \\
      
      
%     % \multicolumn{1}{l}{} & \multicolumn{1}{l}{} & \multicolumn{1}{l}{} &\multicolumn{1}{l}{} &\multicolumn{1}{l}{} &\multicolumn{1}{l}{} &
%     % \multicolumn{1}{l}{} & \multicolumn{1}{l}{} & \multicolumn{1}{l}{} & \multicolumn{1}{l}{} & \multicolumn{1}{l}{} & \multicolumn{1}{l}{}\\[-0.95em] 
    
%     \hline
% \end{tabular}}%

% \caption{Comparison of \ourapproach \ to related for optimization when environmental changes occur.}
% %\lk{Could you add references after all tool names please?}}
% \label{tab:related_work}
% \end{figure*}


\begin{table}[ht]
\centering
\caption{Hardware configuration options.}
\begin{tabular}{lll}
\hline
Configuration Options & Option Values/Range \\
\hline 
\textsf{num\_cores}           &   1 - 4              \\
\textsf{cpu\_frequency}           &  0.3 - 2.0 (GHz)              \\
\textsf{gpu\_frequency}           &  0.1 - 1.3 (GHz)               \\
\textsf{emc\_frequency}           &  0.1 - 1.8 (GHz)               \\
\hline
\end{tabular}
\label{tab:hw_conf}
\end{table}

\begin{table}[ht]
\centering
\caption{Linux OS/Kernel configuration options.}
\resizebox{\linewidth}{!}{
\begin{tabular}{lll}
\hline
Configuration Options & Option Values/Range  \\
\hline 
\textsf{vm.vfs\_cache\_pressure}& 1, 100, 500                 \\  
\textsf{vm.swappiness} &  10, 60, 90\\
\textsf{vm.dirty\_bytes} &30, 60\\
\textsf{vm.dirty\_background\_ratio}&10, 80\\
\textsf{vm.dirty\_background\_bytes}&30, 60\\
\textsf{vm.dirty\_ratio}&5, 10, 20, 50\\
\textsf{vm.nr\_hugepages}&0, 1, 2\\
\textsf{vm.overcommit\_ratio}&50, 80\\
\textsf{vm.overcommit\_memory}&0, 2\\
\textsf{vm.overcommit\_hugepages}&0, 1, 2\\
\textsf{kernel.cpu\_time\_max\_percent}&10 - 100\\
\textsf{kernel.max\_pids}&32768, 65536\\
\textsf{kernel.numa\_balancing} &0, 1\\
\textsf{kernel.sched\_latency\_ns} &24000000, 48000000\\
\textsf{kernel.sched\_nr\_migrate} &32, 64, 128\\
\textsf{kernel.sched\_rt\_period\_us} &1000000, 2000000&\\
\textsf{kernel.sched\_rt\_runtime\_us} &500000, 950000\\
\textsf{kernel.sched\_time\_avg\_ms} &1000, 2000\\
\textsf{kernel.sched\_child\_runs\_first} &0, 1&\\
\textsf{swap\_memory}&1, 2, 3, 4 (GB)\\
\textsf{scheduler.policy}&CFP, NOOP\\
\textsf{drop\_caches}&0, 1, 2, 3\\


\hline
\end{tabular}}
\label{tab:os_conf}
\end{table}


\begin{table}[ht]
\centering
\caption{Configuration options in \textsc{Mlperf Object Detection}, and \textsc{Speech Recongition} software system.}
\begin{tabular}{lll}
\hline
Configuration Options & Option Values/Range  \\
\hline 
\textsf{memory\_growth}                      &    -1, 0.5, 0.9            \\ 
\textsf{logical\_devices}                      &  0, 1               \\ 
\textsf{inter\_op\_parallelism\_threads}& 1, num cpus\\
\textsf{intra\_op\_parallelism\_threads}& 1, num cpus\\
\hline
\end{tabular}
\label{tab:ml_conf}
\end{table}


\begin{table}[ht]
\centering
\caption{Configuration options in \textsc{NLP} software system.}
\begin{tabular}{lll}
\hline
Configuration Options & Option Values/Range  \\
\hline 
\textsf{precision}                      &   8,16           \\ 
\textsf{distributed\_backend}                      &  ddp, dp               \\ 
\textsf{num\_workers}                      &  0, num gpus, 4$\times$ num gpus               \\ 
\hline
\end{tabular}
\label{tab:ml_conf}
\end{table}

\begin{table}[ht]
\centering
\caption{\textsc{Deepstream} software configuration options.}
\resizebox{\linewidth}{!}{
\begin{tabular}{llll}
\hline
Component&Configuration Options & Option Values/Range  \\
\hline 
&\textsf{CRF} &  13, 18, 24, 30               \\  
&\textsf{bitrate} & 1000, 2000, 2800, 5000         \\  
&\textsf{buffer\_size} &  6000, 8000, 20000          \\  
Decoder&\textsf{presets} &   ultrafast, veryfast, faster\\
&& medium, slower  \\  
&\textsf{maximum\_rate} &       600k, 1000k         \\  
&\textsf{refresh} &       OFF, ON         \\  
\hline
&\textsf{batch\_size} &       0 - 30         \\  
&\textsf{batched\_push\_timeout}&  0 - 20           \\  
&\textsf{num\_surfaces\_per\_rame} & 1, 2, 3, 4\\
Stream Mux&\textsf{enable\_padding} & 0, 1          \\  
&\textsf{buffer\_pool\_size} &  1 - 26               \\  
&\textsf{sync\_inputs} &  0, 1          \\ 
&\textsf{nvbuf\_memory\_type} &     0, 1, 2, 3         \\ 
\hline
&\textsf{net\_scale\_factor} &  0.01 - 10              \\  
&\textsf{batch\_size}& 1 - 60                \\  
&\textsf{interval} &  1 - 20               \\  
&\textsf{offset} &       0, 1          \\  
Nvinfer&\textsf{process\_mode} &   0, 1              \\ 
&\textsf{use\_dla\_core} &      0, 1           \\ 
&\textsf{enable\_dla} &           0, 1      \\ 
&\textsf{enable\_dbscan} &       0, 1       \\ 
&\textsf{secondary\_reinfer\_interval} &       0 - 20          \\ 
&\textsf{maintain\_aspect\_ratio} &       0, 1          \\ 
\hline
&\textsf{iou\_threshold} &       0 - 60          \\
&\textsf{enable\_batch\_process} &       0, 1          \\
Nvtracker&\textsf{enable\_past\_frame} &       0, 1          \\
&\textsf{compute\_hw} &       0, 1, 2, 3, 4          \\ 
\hline
\end{tabular}}
\label{tab:deepstream_conf}
\end{table}

\begin{table}[ht]
\centering
\caption{\textsc{Cassandra} configuration options.}
\resizebox{\linewidth}{!}{
\begin{tabular}{lll}
\hline
Configuration Options & Option Values/Range  \\
\hline 
\textsf{concurrent\_writes}& 32, 128, 512                  \\  
\textsf{file\_cache\_size} &  256, 512, 2048\\
\textsf{memtable\_cleanup} &0.1, 0.3, 0.6\\
\textsf{concurrent\_compact} &0.1, 0.3, 0.6\\
\textsf{compaction\_methods} &SizeTiered, LeveledCompaction\\
\textsf{num\_tokens} &256, 512, 1024\\
\textsf{concurrent\_reads} &32, 64, 128\\
\textsf{replication\_factor} &1, 2, 3\\
\textsf{memtable\_heap\_space} &256, 1024, 2048\\
\textsf{memtable\_allocation} &heap, buffers\\
\textsf{row\_cache\_size\_in\_mb} &0, 1\\
\textsf{sstable\_open\_interval} &30, 50, 100\\
\textsf{trickle\_fsync} & 0, 1\\
\textsf{inter\_dc\_stream} &100, 200\\
\textsf{key\_cache\_ssize} &100, 200\\
\textsf{stream\_throughput} &100, 200\\
\textsf{row\_cache\_save} & 0, 1\\
\textsf{column\_index\_size} &16, 32, 64\\
\textsf{compaction\_throughput} &16, 32, 64\\
\textsf{memtable\_offheap\_space} &256, 1024, 2048\\
\textsf{commitlog\_segment} &32, 64, 256\\
\textsf{mem\_flush\_writers} &1, 2, 3\\
\textsf{index\_summary} &100, 150\\

\hline
\end{tabular}}
\label{tab:os_conf}
\end{table}
\begin{table}[ht]
\centering
\caption{Performance system events and tracepoints. }
\begin{tabular}{lll}
\hline
System Events \\
\hline 
\textsf{context\_switches}\\ 
\textsf{major\_faults}         \\ 
\textsf{minor\_faults}                              \\ 
\textsf{migrations}                           \\ 
\textsf{scheduler\_wait\_time}                             \\ 
\textsf{scheduler\_sleep\_time}                             \\ 
\textsf{cycles}                               \\
\textsf{instructions}                             \\ 
\textsf{number\_of\_syscall\_enter}                       \\ 
\textsf{number\_of\_syscall\_exit}                       \\ 
\textsf{l1\_dcache\_load\_misses}            \\                   
\textsf{l1\_dcache\_loads}                               \\
\textsf{l1\_dcache\_stores}                               \\
\textsf{branch\_loads}                               \\
\textsf{branch\_loads\_misses}                            \\
\textsf{branch\_misses}                            \\
\textsf{cache\_references}\\
\textsf{cache\_misses}\\
\textsf{emulation\_faults}                               \\
% Alignment faults \\
\hline
Tracepoint Subsystems\\
\hline
\textsf{Block}\\
\textsf{Scheduler}\\
\textsf{IRQ}\\
\textsf{ext4}\\
\hline
\end{tabular}
\label{tab:event_conf}
\end{table}

\begin{table}[ht]
\centering
\caption{Hyperparameters for DNNs used in \ourapproach.}
\resizebox{\linewidth}{!}{\begin{tabular}{lll}
\hline
Architecture & Hyperparameters & Option Values\\
\hline 
&\textsf{num\_filters\_entry} flow &32 \\
&\textsf{filter\_size\_entry\_flow} &(3 $\times$ 3)\\
&\textsf{num\_filters\_middle\_flow} &64 \\
&\textsf{filter\_size\_middle\_flow} &(3 $\times$ 3)\\
\textsc{ResNet}&\textsf{num\_filters\_exit\_flow} &728\\
&\textsf{filter\_size\_exit\_flow} &(3 $\times$ 3)\\
&\textsf{batch\_size} &32\\
&\textsf{num\_epochs}&100\\
\hline
&\textsf{dropout} & 0.3\\
&\textsf{maximum\_batch\_size}&16\\
\textsc{Bert}&\textsf{maximum\_sequence\_length}&13\\
&\textsf{learning\_rate} &$1e^{-4}$\\
&\textsf{weight\_decay} &0.3\\
\hline
&\textsf{dropout} & 0.3\\
&\textsf{maximum\_batch\_size}& 16\\
\textsc{Deepspeech}&\textsf{maximum\_sequence\_length}&32\\
&\textsf{learning\_rate} &$1e^{-4}$\\
&\textsf{num\_epochs}&10\\
\hline
\end{tabular}}
\label{tab:dnn_conf}
\end{table}

\begin{figure}[ht]
    \centering
    \includegraphics[width=0.49\textwidth]{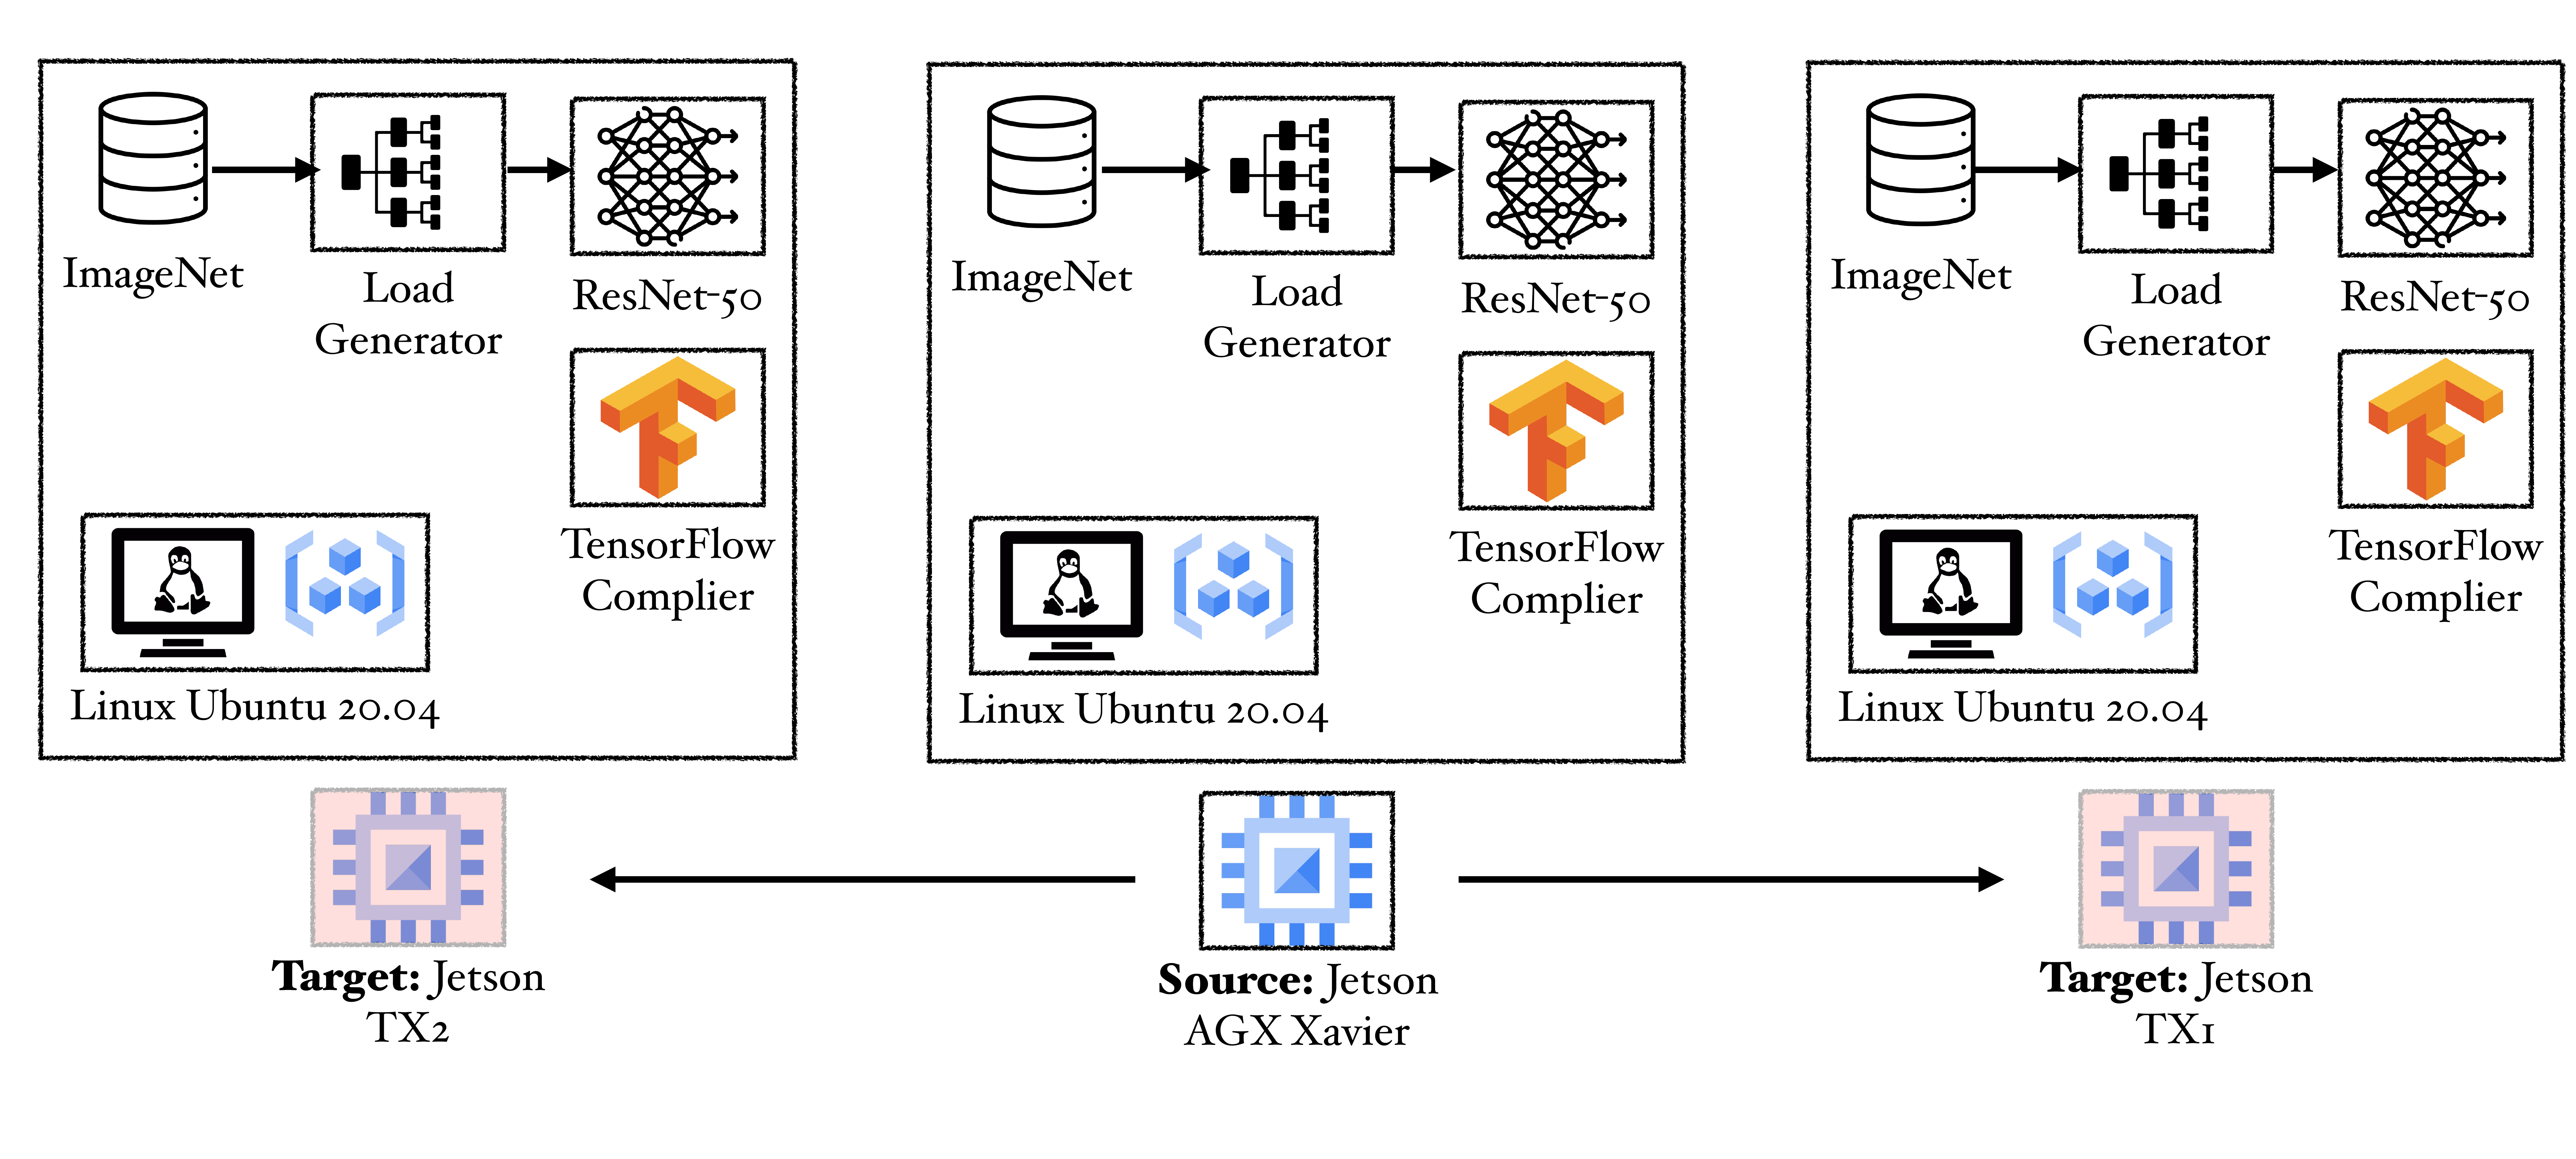}
    \caption{Experimental setup when hardware changes from \xavier in the source to \txtwo and \txone in the target, separately, for \textsc{MlPerf Object Detection} pipeline.}
     \label{fig:hw_change_dep}
\end{figure}

\begin{table}[ht]
% \begin{table}[!]
\centering
\caption{Hyperparameters for FCI used in \ourapproach.}
\begin{tabular}{lll}
\hline
Hyperparameters & Value \\
\hline 
\textsf{depth} &-1 \\
\textsf{test\_id} &fisher-z-test\\
\textsf{maximum\_path\_length} &-1 \\
\textsf{complete\_rule\_set\_used}&False\\
\hline 

\end{tabular}
\label{tab:fci_conf}
\end{table}



\begin{figure}[ht]
    \centering
    \includegraphics[width=0.48\textwidth]{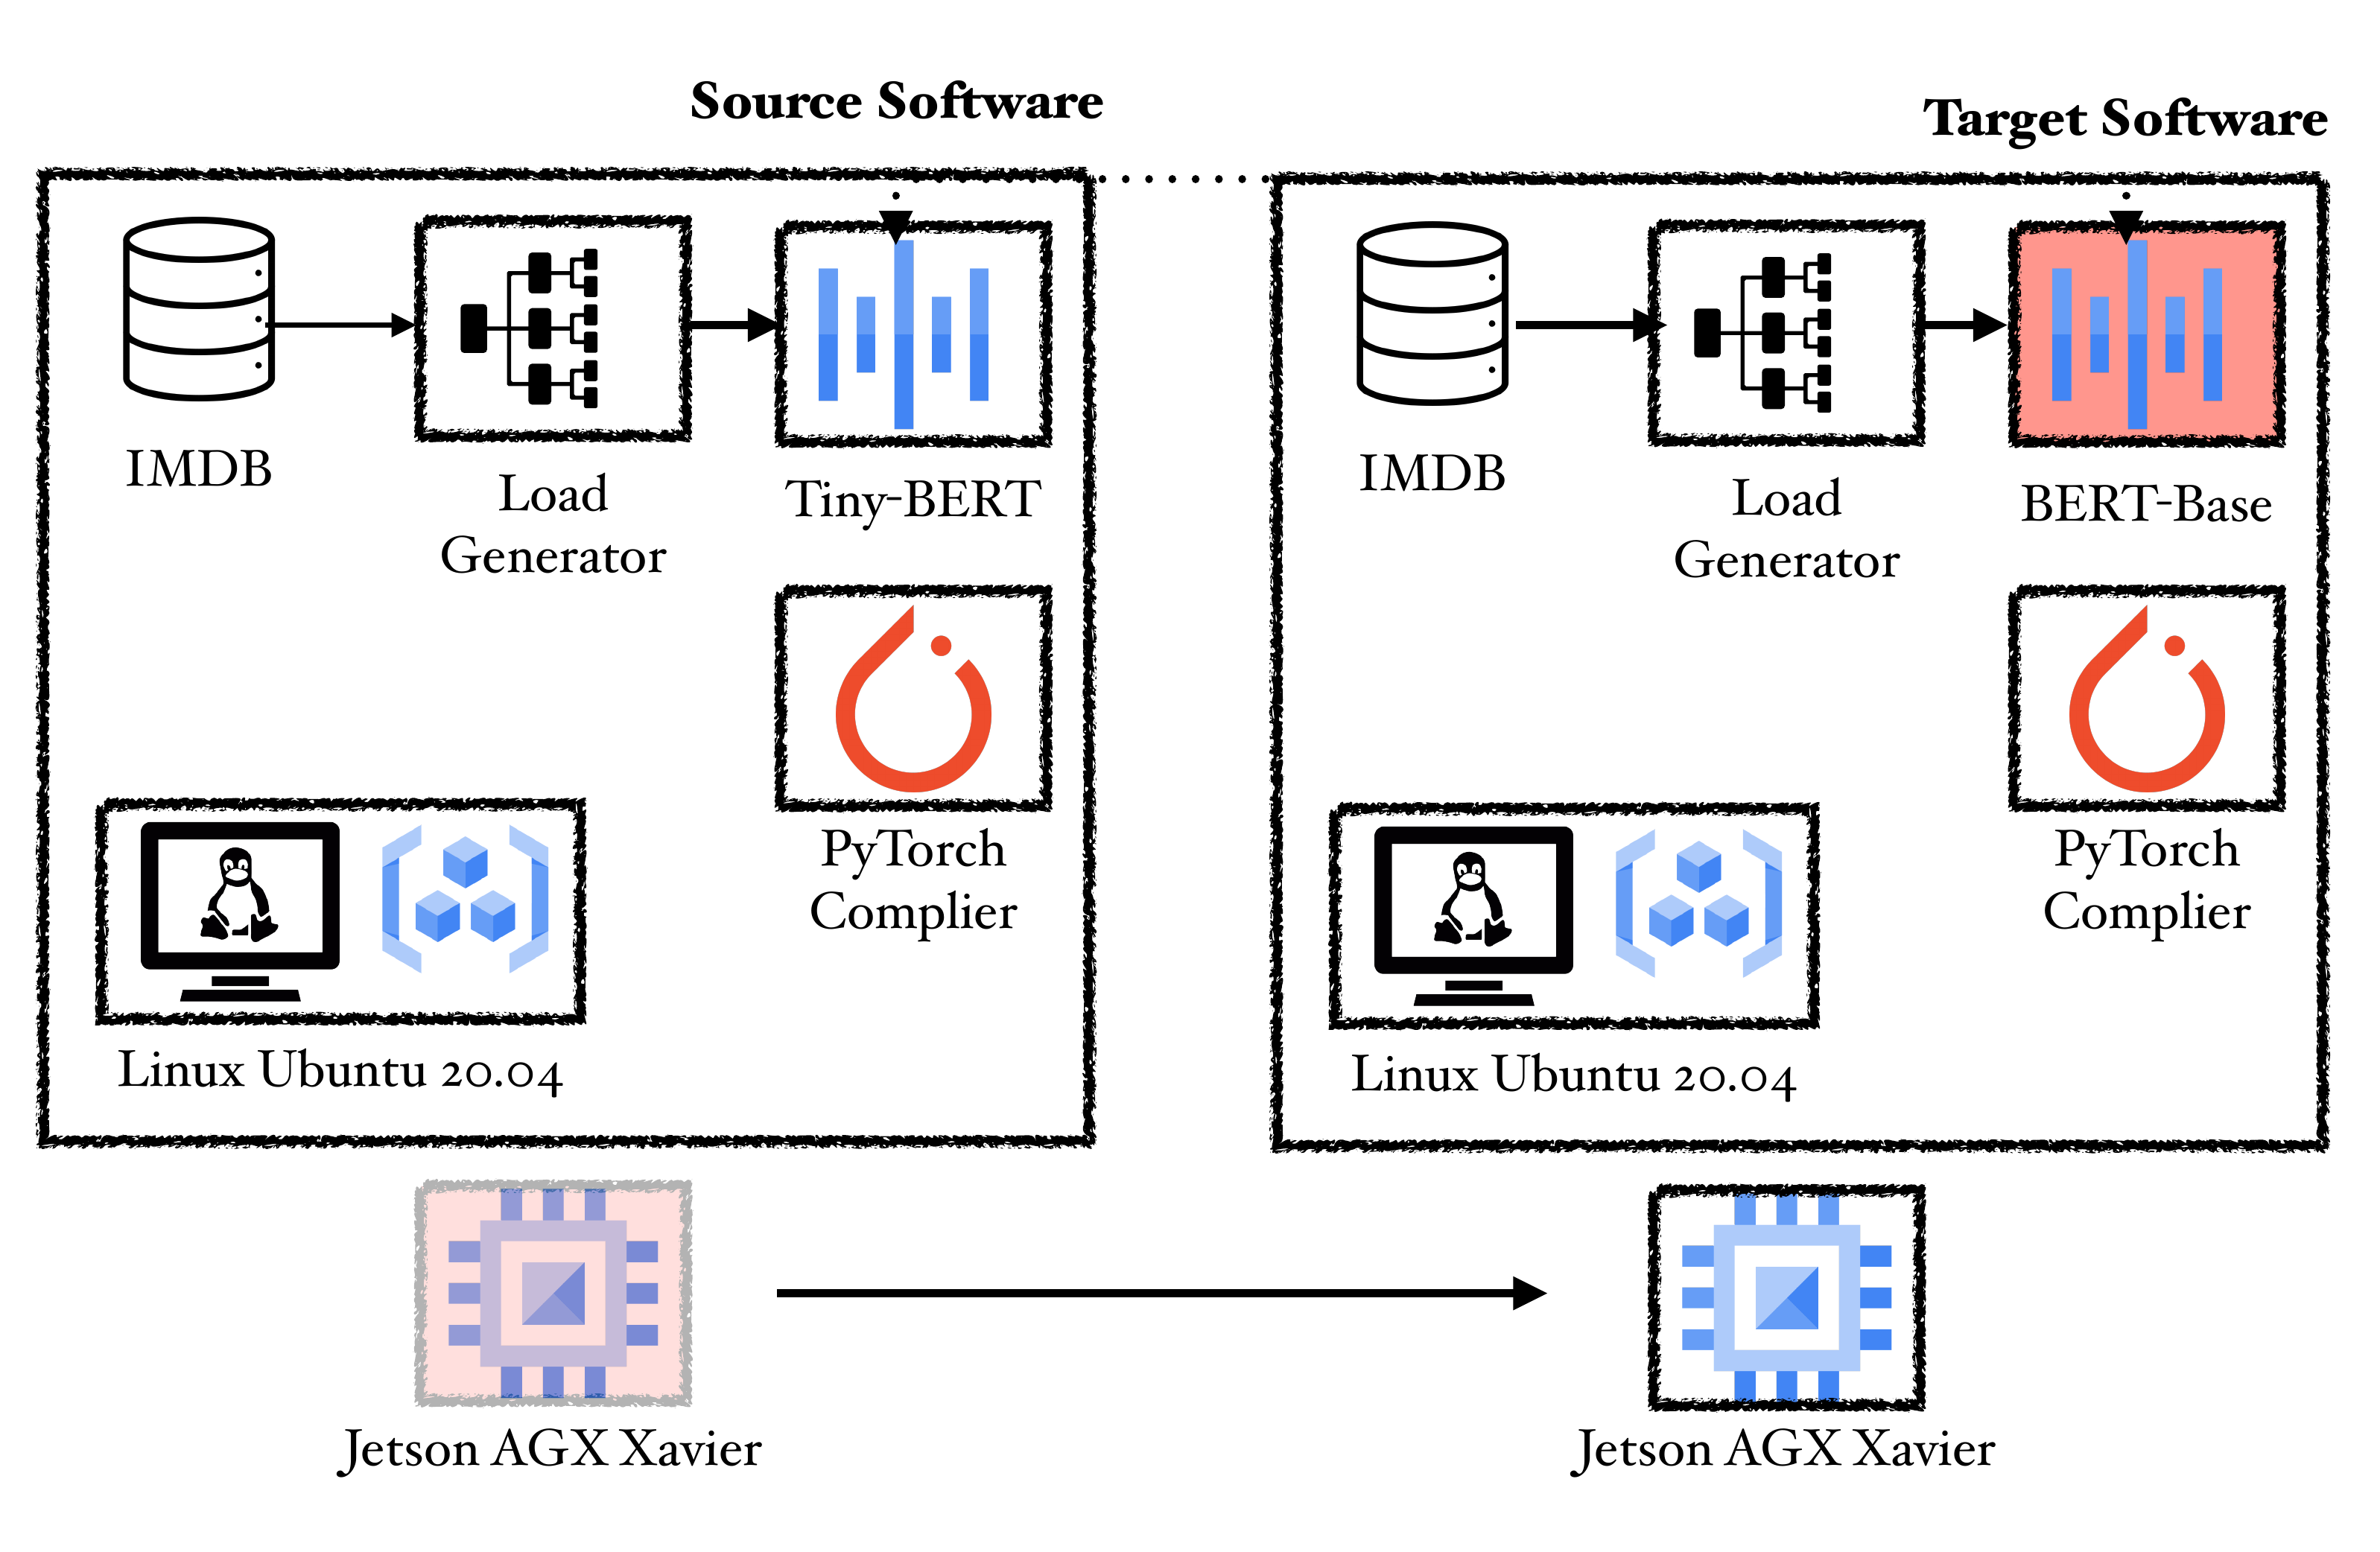}
    \caption{Experimental setup when a software change takes place from {TinyBERT} to {BERT-Base} in the target for a NLP system.}
    \label{fig:software_change_dep}
\end{figure}

\begin{figure}[H]
    \centering
    \includegraphics[width=0.48\textwidth]{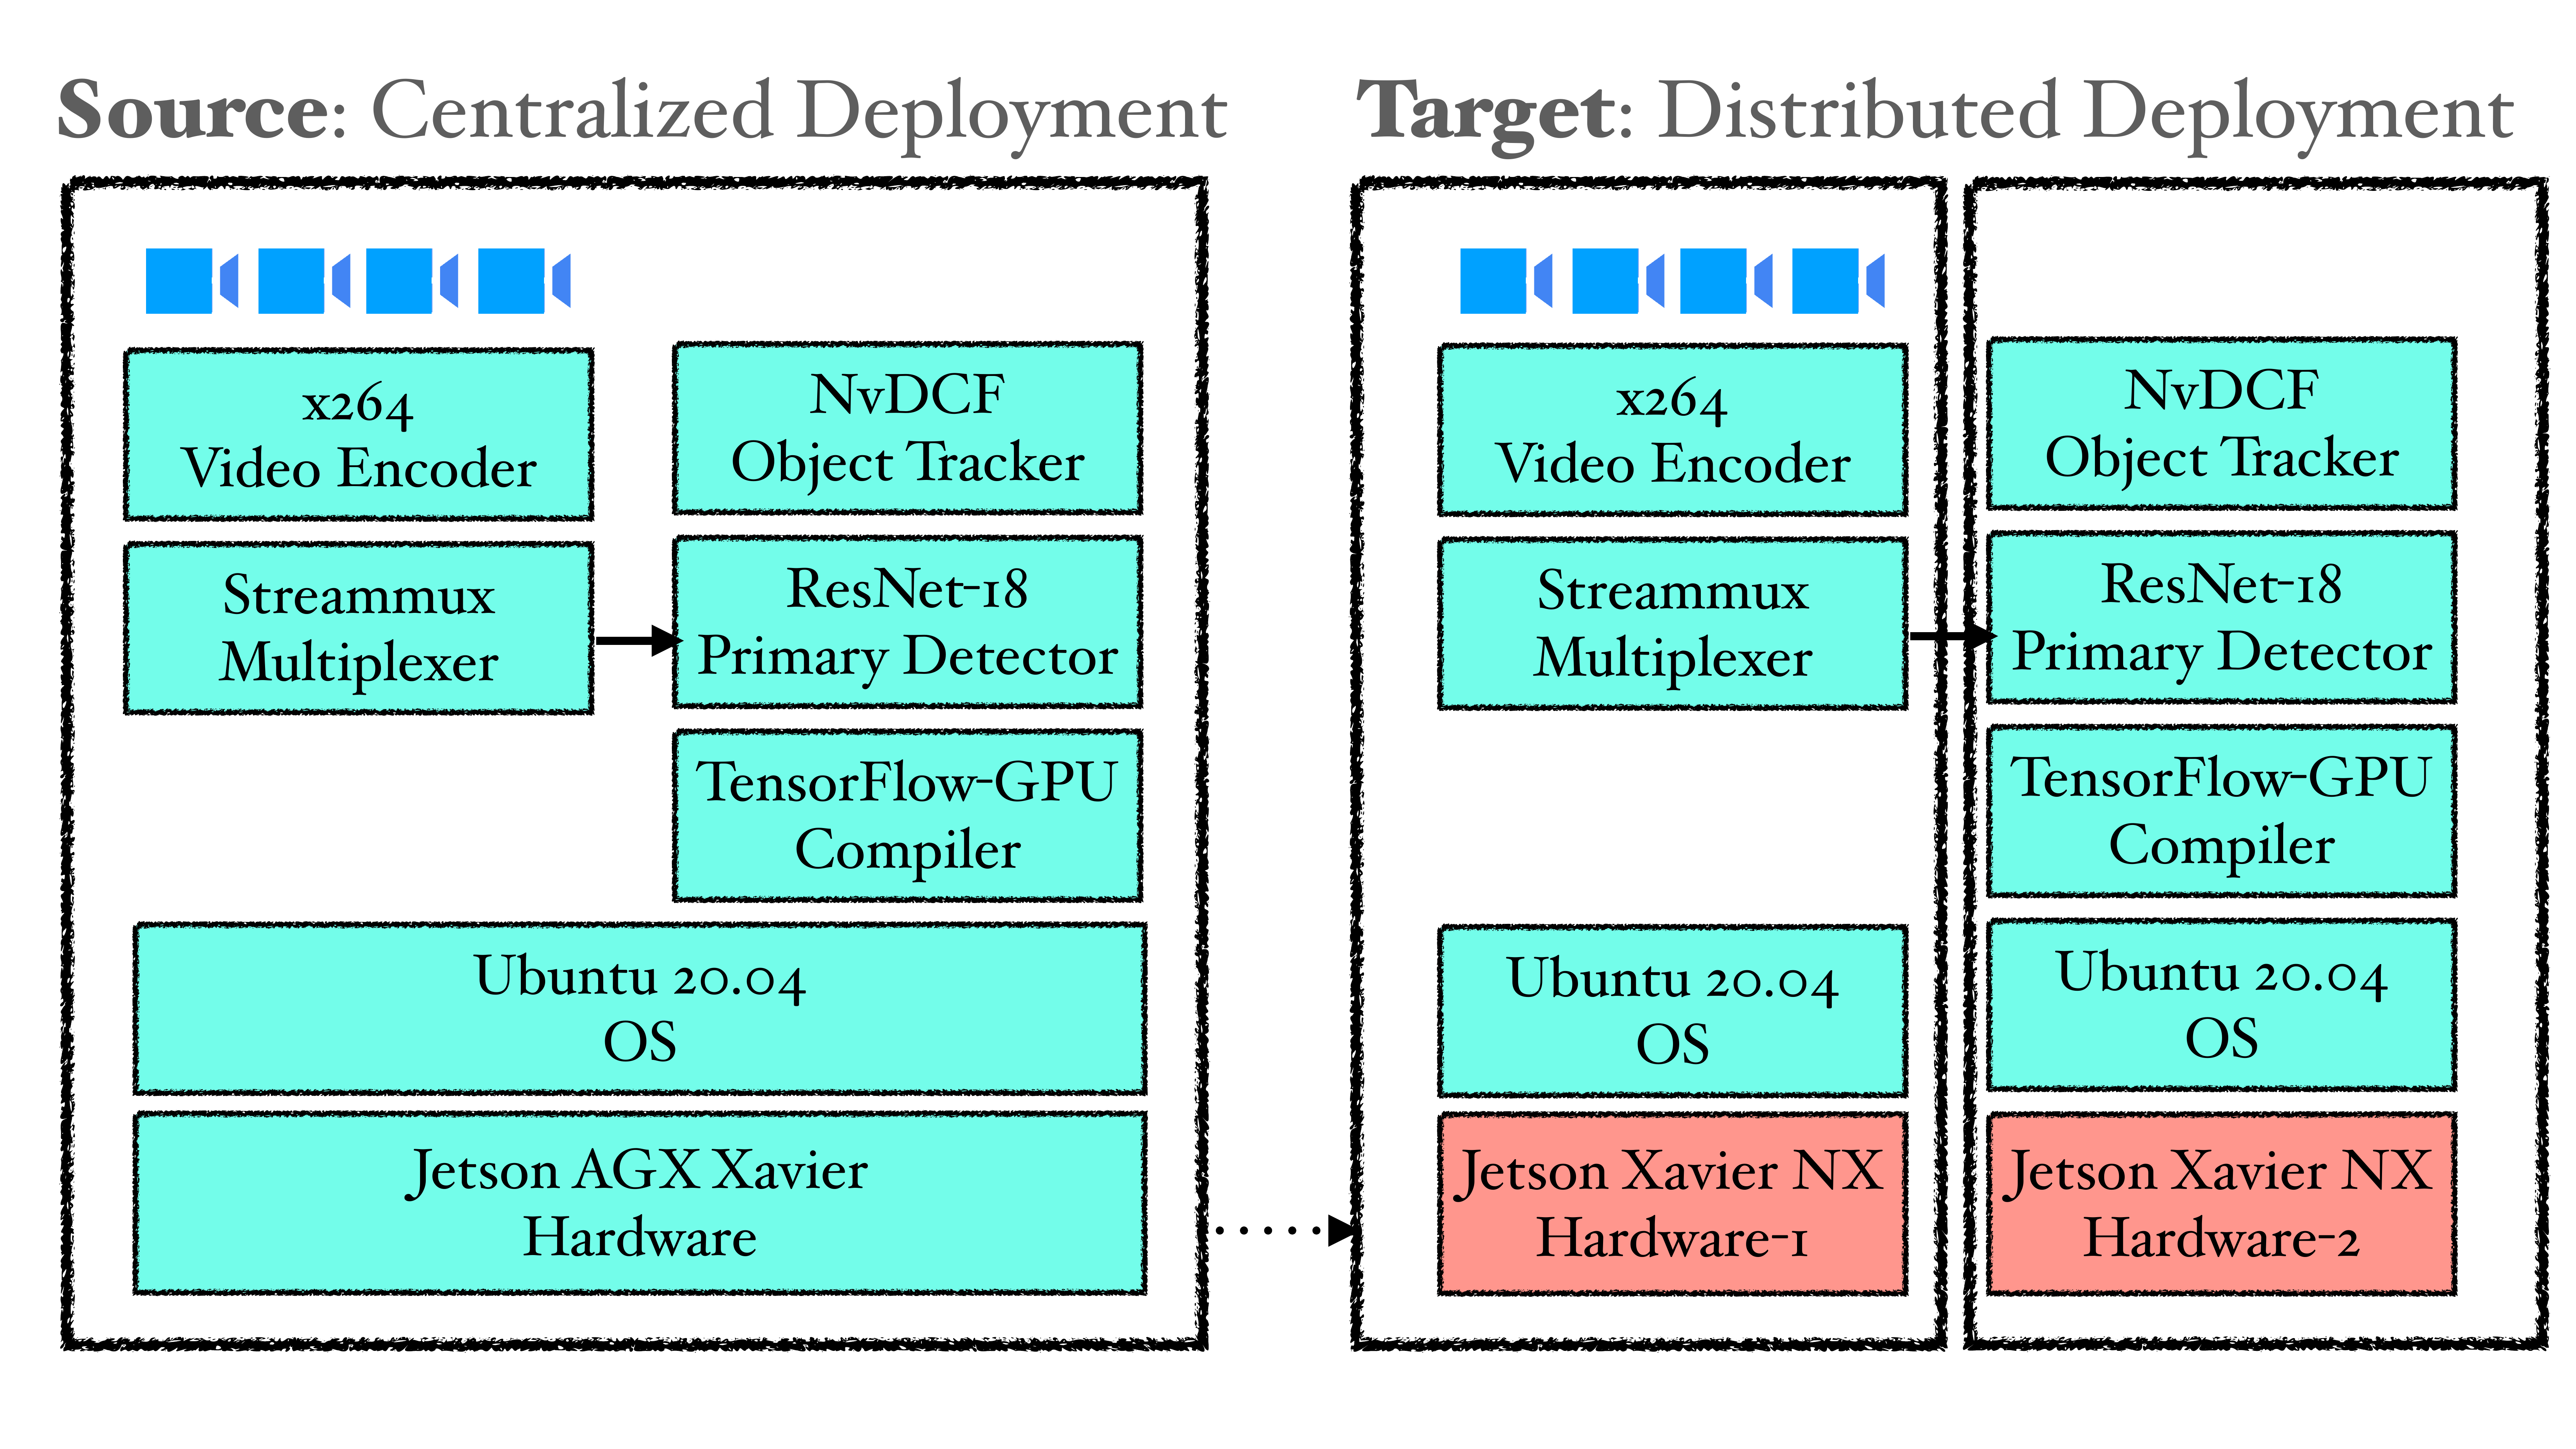}
    \caption{Experimental setup for our experiments when the deployment topology is changed from centralized to distributed in the target in the target using two \xavier NX.}
     \label{fig:deployment_change_dep}
\end{figure}


\begin{figure}[!ht]
    \centering
    \includegraphics[width=0.48\textwidth]{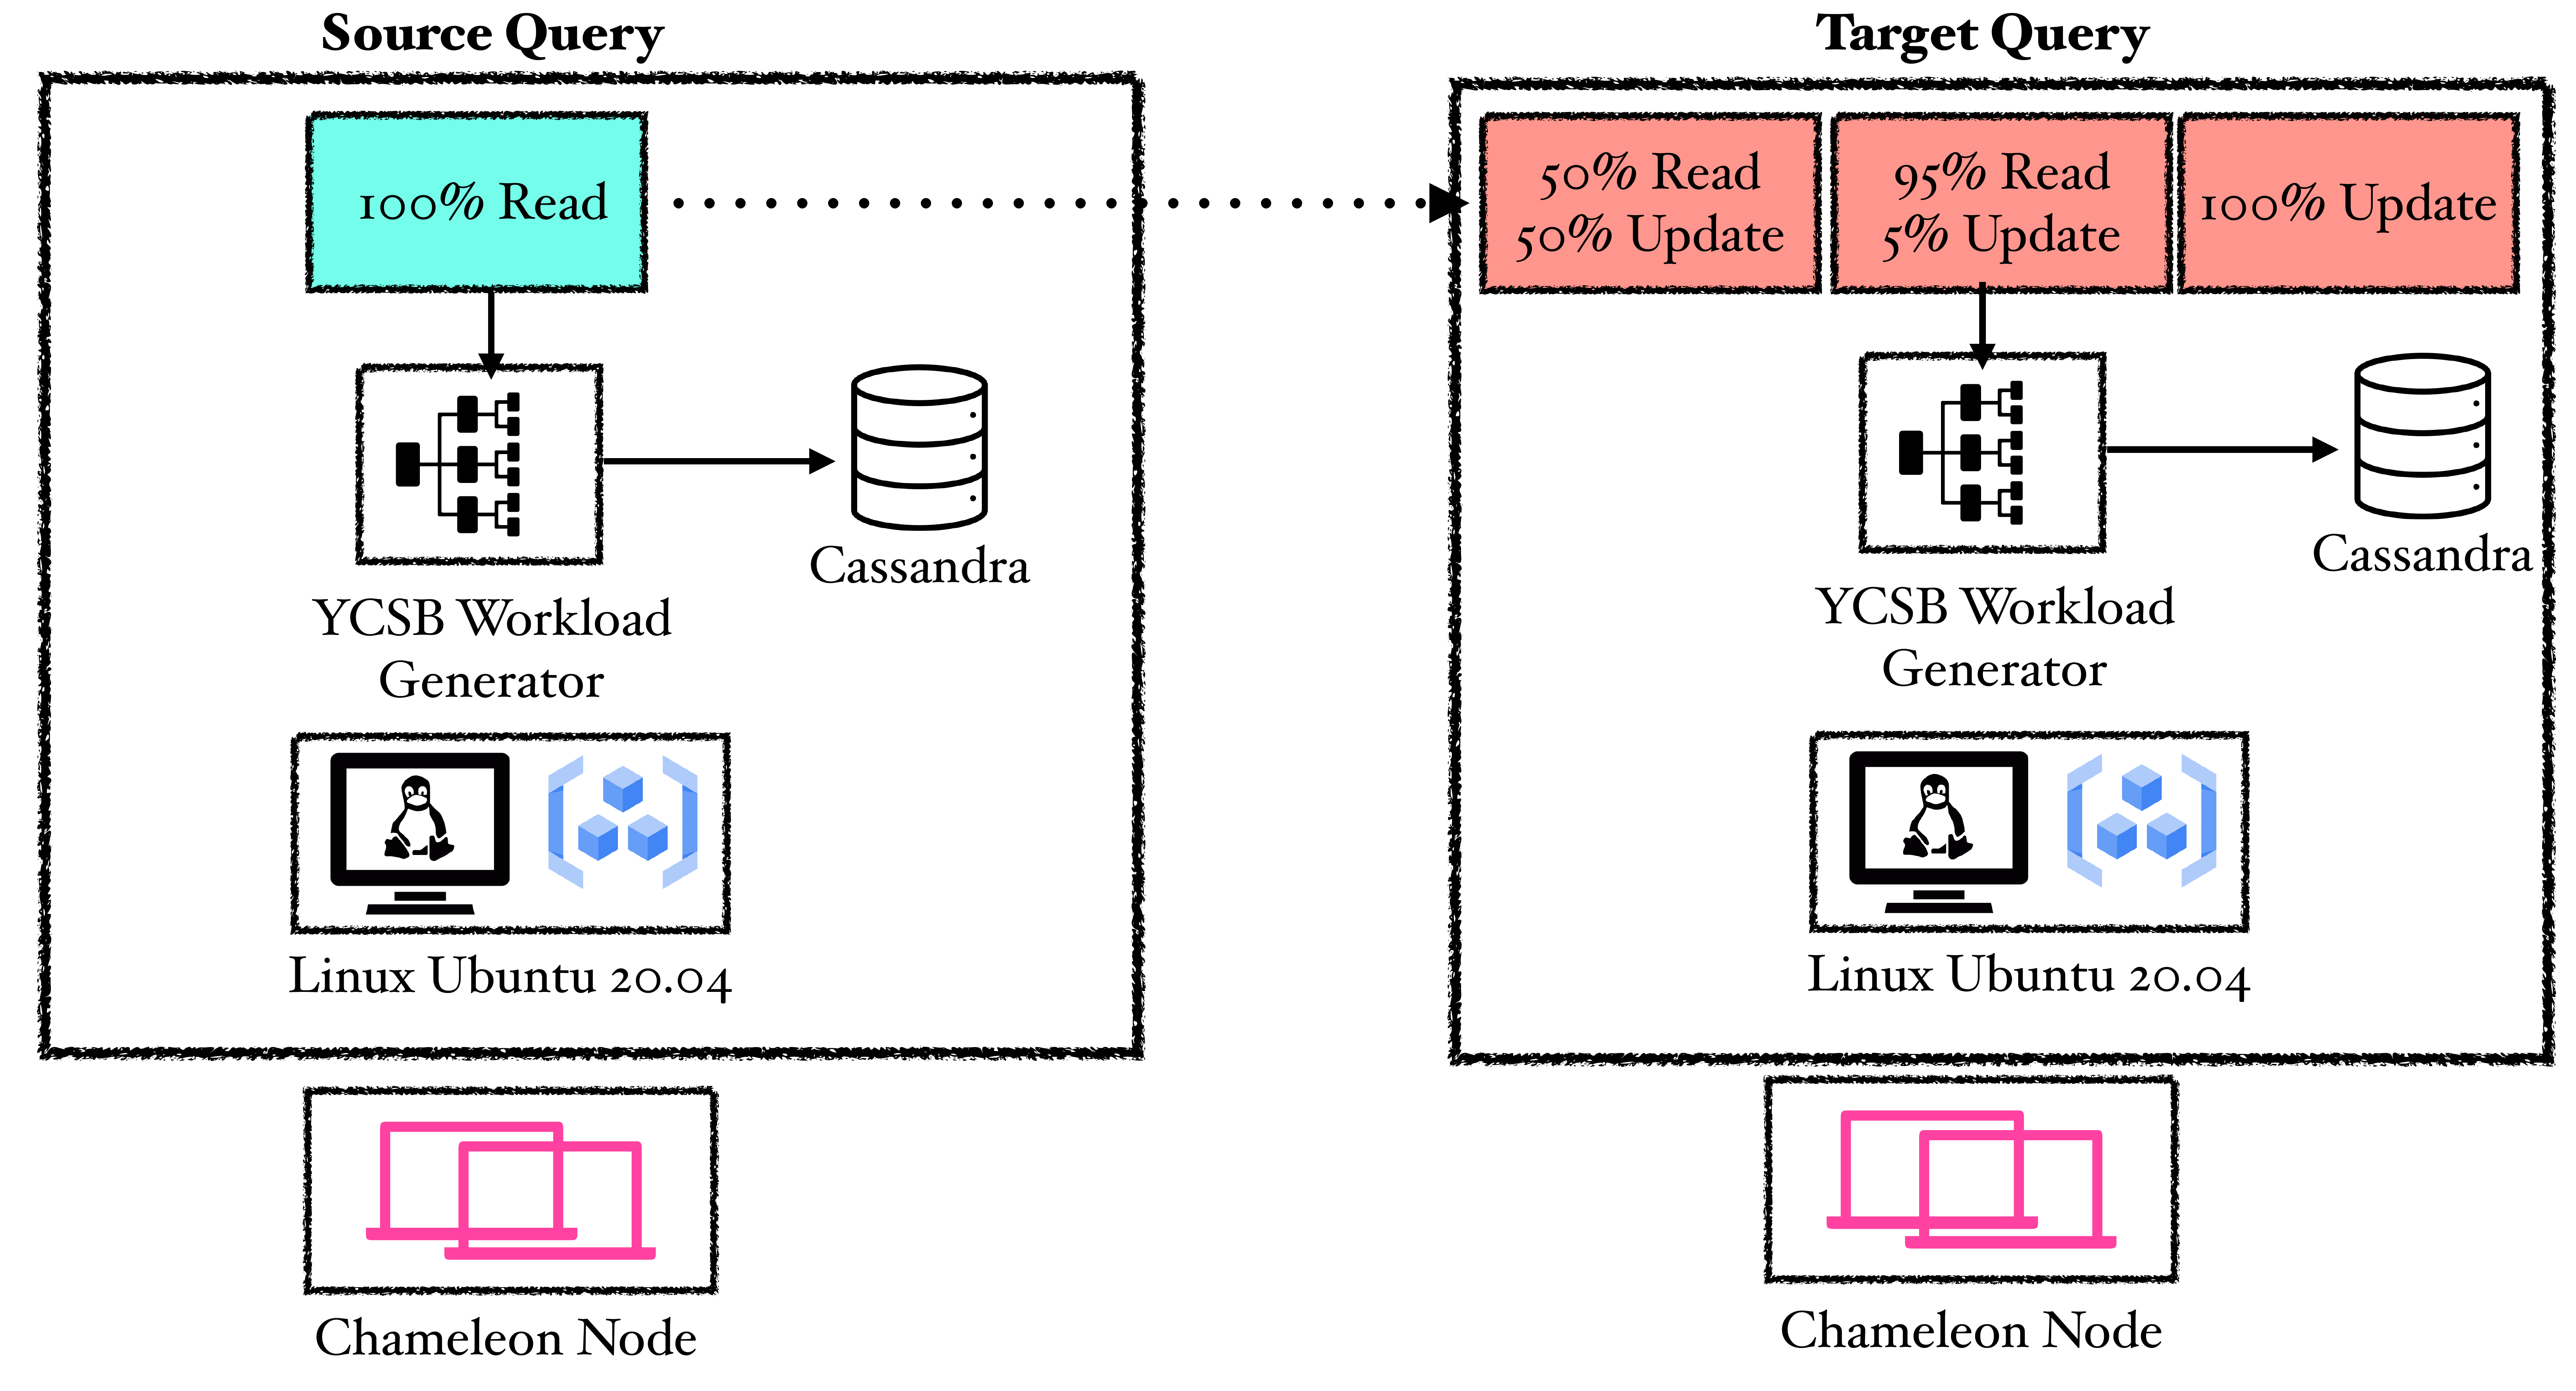}
    \caption{Experimental setup when the type of workload is different with a \textsc{Cassandra} database where the source uses a \textsc{Read Only} workload where the target uses a \textsc{Balanced} and \textsc{Update Heavy} workload, separately. }
     \label{fig:workload_change_dep}
\end{figure}


\begin{figure*}[ht]
    \centering
    \includegraphics[width=\textwidth]{Figures/rq2_env_change.pdf}
    \caption{Experimental setup for different severity of environmental changes. Low serverity of environmental change setup when only hardware changes from \xavier to \xavier NX in the target (second figure). For medium severity environmental change experimental setup, we change the hardware and deployment topology (third figure). For high severity enviornmental changes experiments, the primary detector is changed from \textsc{ResNet-18} to \textsc{ResNet-50}, decoder is changed from \textsc{x264} to \textsc{x265} with a different deployment topology from the source distributed with two \xavier NX hardware that is different from the source as well (fourth figure). }
     \label{fig:severity_change_dep}
\end{figure*}



\subsection{RQ1 Additional Results}
\Cref{tab:optimal_config} shows the best configuration and latency found by each method and the optimal configuration for the features having the highest causal effects. It can be seen that the configuration found by \ourapproach is much closer to the optimal one. The highlighted cells indicate the options which are correctly identified by different method. 
\begin{table*}[]
\scriptsize
\caption{\small{Optimal configuration discovered by different baselines. The configuration options are ranked in descending order based on their average causal effect (ACE) value on the performance objective, i.e., Latency.}}
\centering
\begin{tabular}{cccccccccc}
\hline
Option & \smac & \unicorn & \restune &\restuner&\ourapproach&ACE&Optimal (Source)&Optimal (Target)&Initial (Target)\\
\hline
\textsf{cpu\_frequency}&1.3&1.6&1.6&1.6&\cellcolor{red!20}2.0&0.19&1.4&\cellcolor{red!20}2.0&1.1\\
\textsf{vm.dirty\_ratio}&20&\cellcolor{red!20}5&20&\cellcolor{red!20}5&\cellcolor{red!20}5&0.13&10&\cellcolor{red!20}5&50\\
\textsf{vm.swappiness}&\cellcolor{red!20}60&\cellcolor{red!20}60&\cellcolor{red!20}60&\cellcolor{red!20}60&\cellcolor{red!20}60&0.11&30&\cellcolor{red!20}60&30\\
\textsf{gpu\_frequency}&\cellcolor{red!20}1.3&\cellcolor{red!20}1.3&\cellcolor{red!20}1.3&\cellcolor{red!20}1.3&\cellcolor{red!20}1.3&0.08&1.3&\cellcolor{red!20}1.3&1.1\\
\textsf{num\_cores}&3&\cellcolor{red!20}4&3&\cellcolor{red!20}4&\cellcolor{red!20}4&0.06&3&\cellcolor{red!20}4&2\\
\textsf{memory\_growth}&0.5&0.9&0.5&0.9&\cellcolor{red!20}-1&0.04&0.5&\cellcolor{red!20}-1&0.5\\
\textsf{emc\_frequency}&1.1&\cellcolor{red!20}1.3&\cellcolor{red!20}1.3&1.1&\cellcolor{red!20}1.3&0.009&1.1&\cellcolor{red!20}1.3&0.8\\
\textsf{drop\_caches}&\cellcolor{red!20}0&\cellcolor{red!20}0&\cellcolor{red!20}0&\cellcolor{red!20}0&\cellcolor{red!20}0&0.008&0&\cellcolor{red!20}0&1\\
\textsf{scheduler\_policy}&\cellcolor{red!20}NOOP&\cellcolor{red!20}NOOP&CFP&\cellcolor{red!20}NOOP&\cellcolor{red!20}NOOP&0.001&NOOP&\cellcolor{red!20}NOOP&CFP\\
\textsf{vm.vfs\_cache\_pressure}&10&50&10&10&10&0.001&10&10&50\\
\textsf{vm.dirty\_bytes}&\cellcolor{red!20}30&60&60&\cellcolor{red!20}30&60&0.0009&30&\cellcolor{red!20}30&60\\
\textsf{kernel.sched\_rt\_runtime\_us}&500000&500000&500000&500000&\cellcolor{red!20}950000&0.0009&500000&\cellcolor{red!20}9500000&500000\\
\textsf{logical\_devices}&\cellcolor{red!20}1&\cellcolor{red!20}1&\cellcolor{red!20}0&\cellcolor{red!20}1&\cellcolor{red!20}1&0.0008&1&\cellcolor{red!20}1&0\\
\textsf{kernel.sched\_child\_runs\_first}&\cellcolor{red!20}0&\cellcolor{red!20}0&\cellcolor{red!20}0&\cellcolor{red!20}0&\cellcolor{red!20}0&0.0006&0&\cellcolor{red!20}0&1\\
Latency&19s&17s&18s&14s&11s&&23s&9s&48s\\

\hline
\end{tabular}
\label{tab:optimal_config}
\vspace{-3mm}
\end{table*}

\Cref{tab:ml_conf} shows the detailed model computational time and total time (including both model computational time and the configuration evaluation time) per iteration.

\begin{table}[ht]
\scriptsize
\centering
\caption{\small{Comparison of computation time in seconds required per iteration for different baselines when compared to \ourapproach. Lower is better.}}
\resizebox{.48\textwidth}{!}{
\begin{tabular}{cccc}
\hline
Method & Model Update & Configuration& Total \\
& Time & Recommendation Time & Time\\
\hline 
\smac  & \cellcolor{red!20}5.6 & \cellcolor{red!20}9.2 & \cellcolor{red!20}58.1           \\
\cello  & 8.1 & \cellcolor{red!20}9.2 & 60.3          \\ 
\unicorn  & 11.5 & 11.3 & 65.4          \\
\restune  & 8.3 & \cellcolor{red!20}9.2 & 61.3          \\
\restuner  & 9.7 & 9.7 & 63.4          \\
\hline
\ourapproach & 12.7 & 14.4 & 71.6          \\

\hline
\end{tabular}}
\label{tab:ml_conf}
\end{table}

\begin{table}
\centering
\scriptsize
\caption{\small{Constrained optimization results for latency with energy constraint and energy with latency constraint averaged over difference percentiles.}}
\resizebox{.45\textwidth}{!}{
\begin{tabularx}{0.52\textwidth}{c|ccc|ccc}
    \toprule
\multirow{2}{*}{Environment} 
        & \multicolumn{3}{c}{Latency Under Energy (RE\%)} & \multicolumn{3}{c}{Energy Under Latency (RE\%)}   \\
    \cmidrule(lr){2-4} \cmidrule(lr){5-7}
        Change & \cello  & \unicorn  & \ourapproach  & \cello  & \unicorn  & \ourapproach          \\
    \midrule
\multirow{1}{*}{Hardware} 
  & 16.8  & 13.6  & \cellcolor{red!20}9.7  & 14.1  & 15.2  & \cellcolor{red!20}13.9\\
      
       
       \multirow{1}{*}{Software}  
        & 17.1  & 19.2  & \cellcolor{red!20}22.5  & 30.9  & 31.5  &\cellcolor{red!20}23.7 \\
             
       \multirow{1}{*}{Workload}  
        & \cellcolor{red!20}9.5  & 11.2  & 9.6  & 14.7  & 13.2  & \cellcolor{red!20}11.1 \\
         
       \multirow{1}{*}{Deployment}  
        & 14.3  & 13.3  & \cellcolor{red!20}11.4  & 18.1  & 16.7  & \cellcolor{red!20}11.3 \\
 \hline

\end{tabularx}
}
\end{table}

\begin{figure}[ht]
  \centering
  \includegraphics[width=0.48\columnwidth]{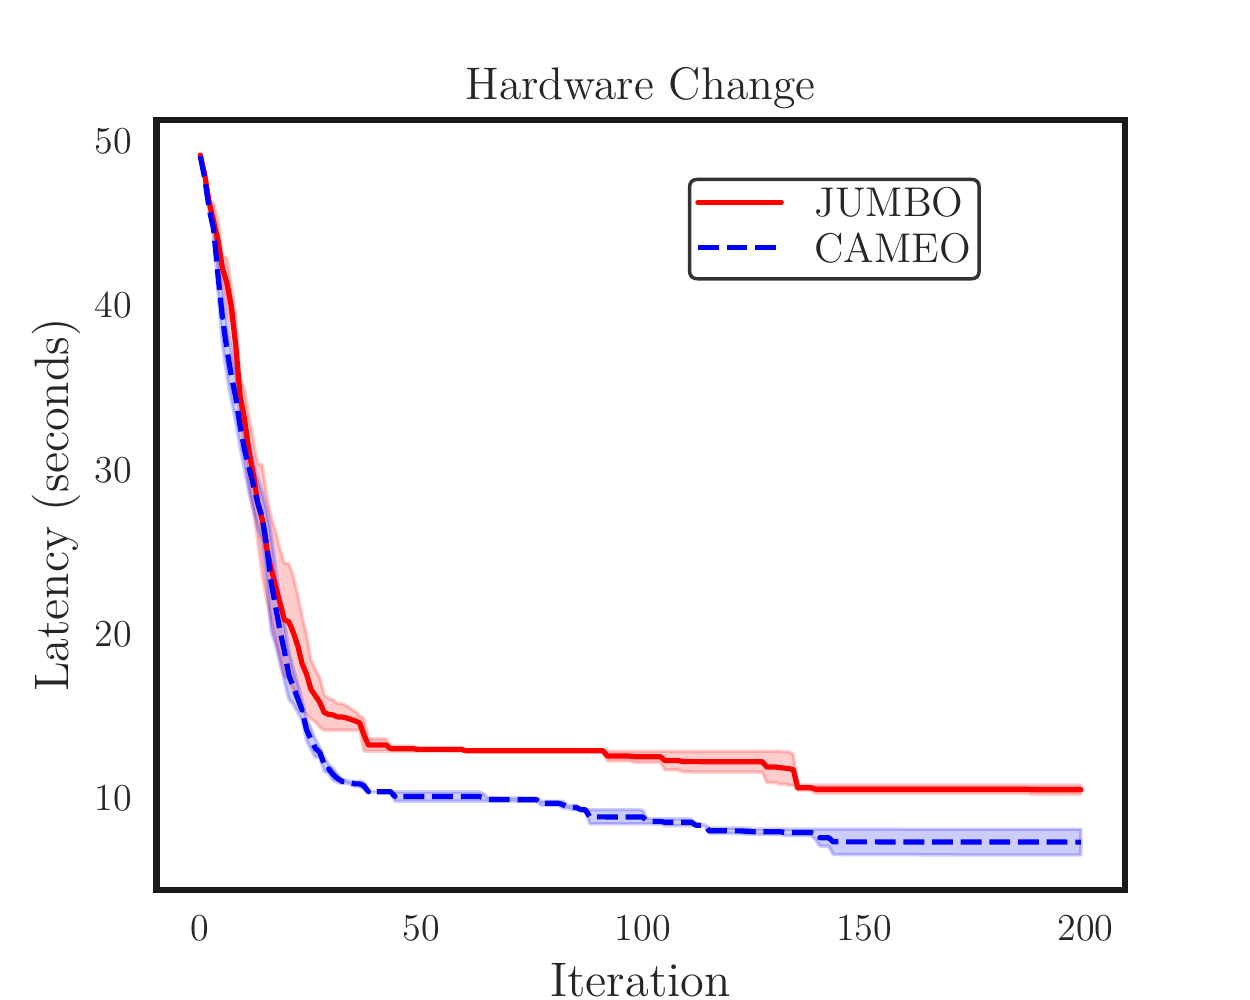}
  \includegraphics[width=0.48\columnwidth]{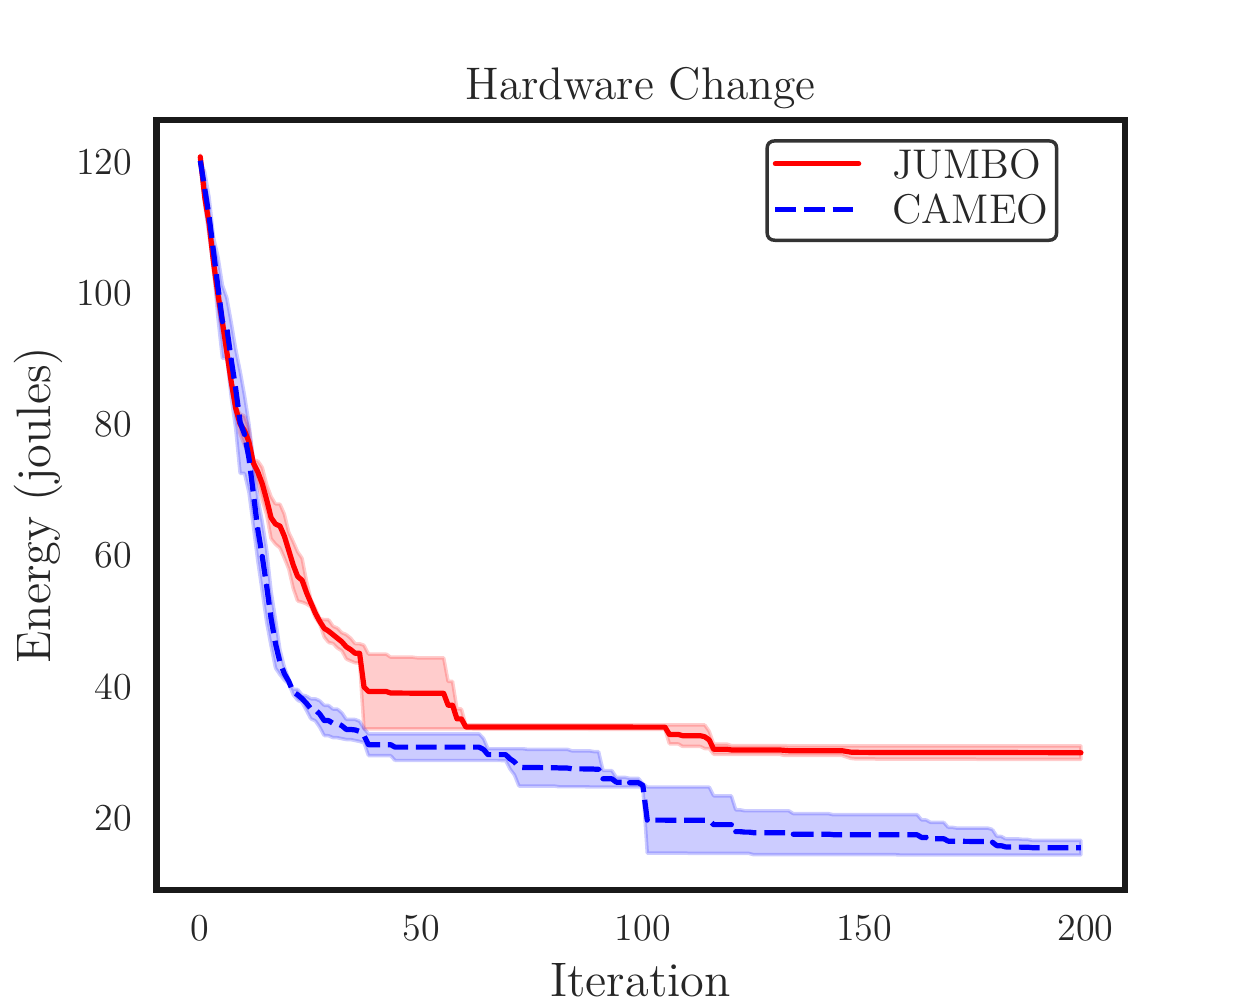}
  
%   \includegraphics[width=0.3\textwidth]{Figures/rq1_model_latency.pdf}
%   \includegraphics[width=0.3\textwidth]{Figures/rq1_workload_latency.pdf}
  \caption{\small{Effectiveness of \ourapproach when hardware changes in the deployment environment.}}
   \label{fig:rq1_app_hw}
\vspace{-3mm}
\end{figure}

\begin{figure}[ht]
  \centering
  \includegraphics[width=0.48\columnwidth]{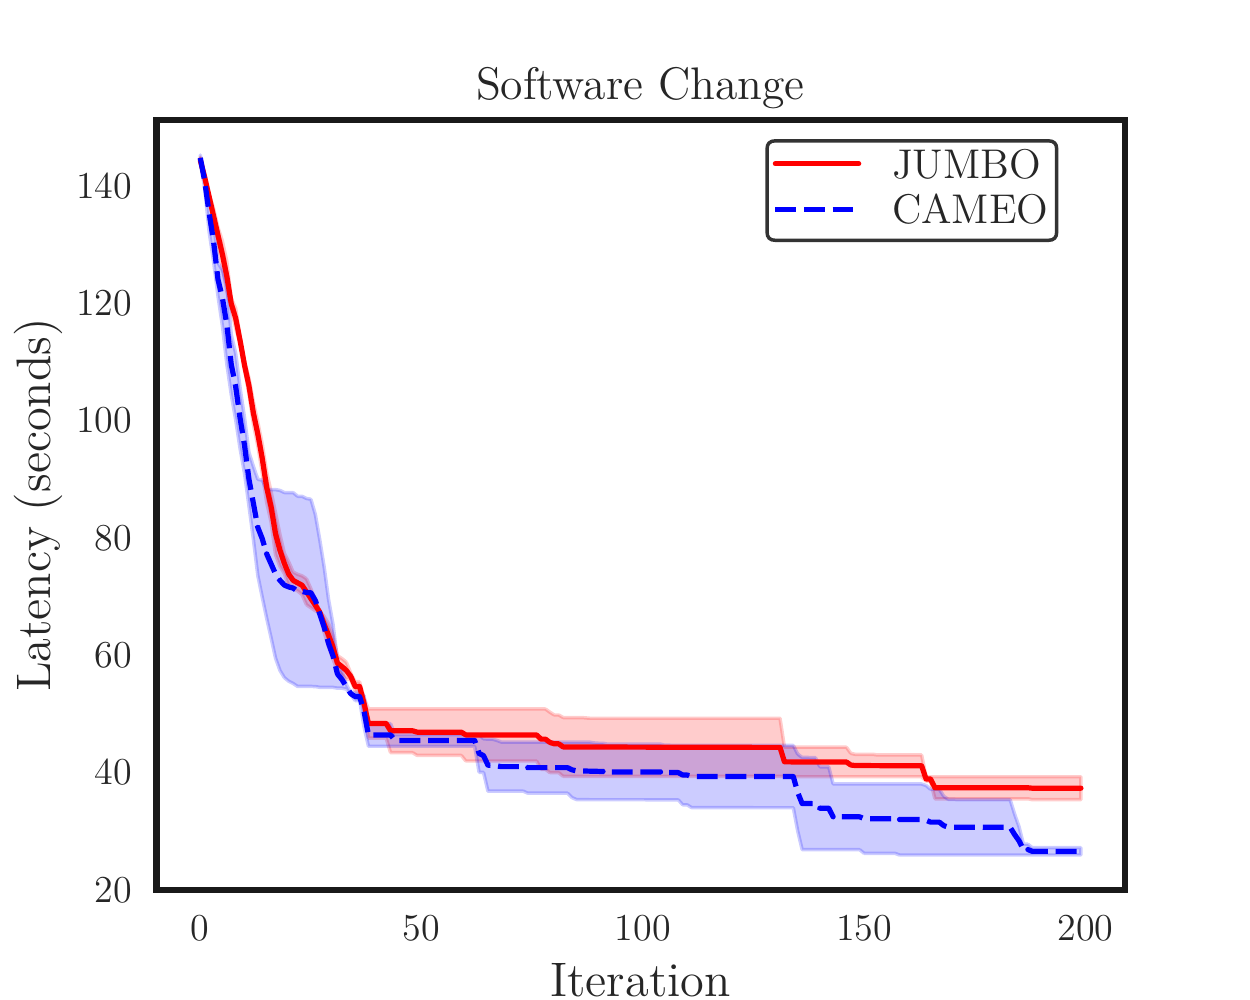}
  \includegraphics[width=0.48\columnwidth]{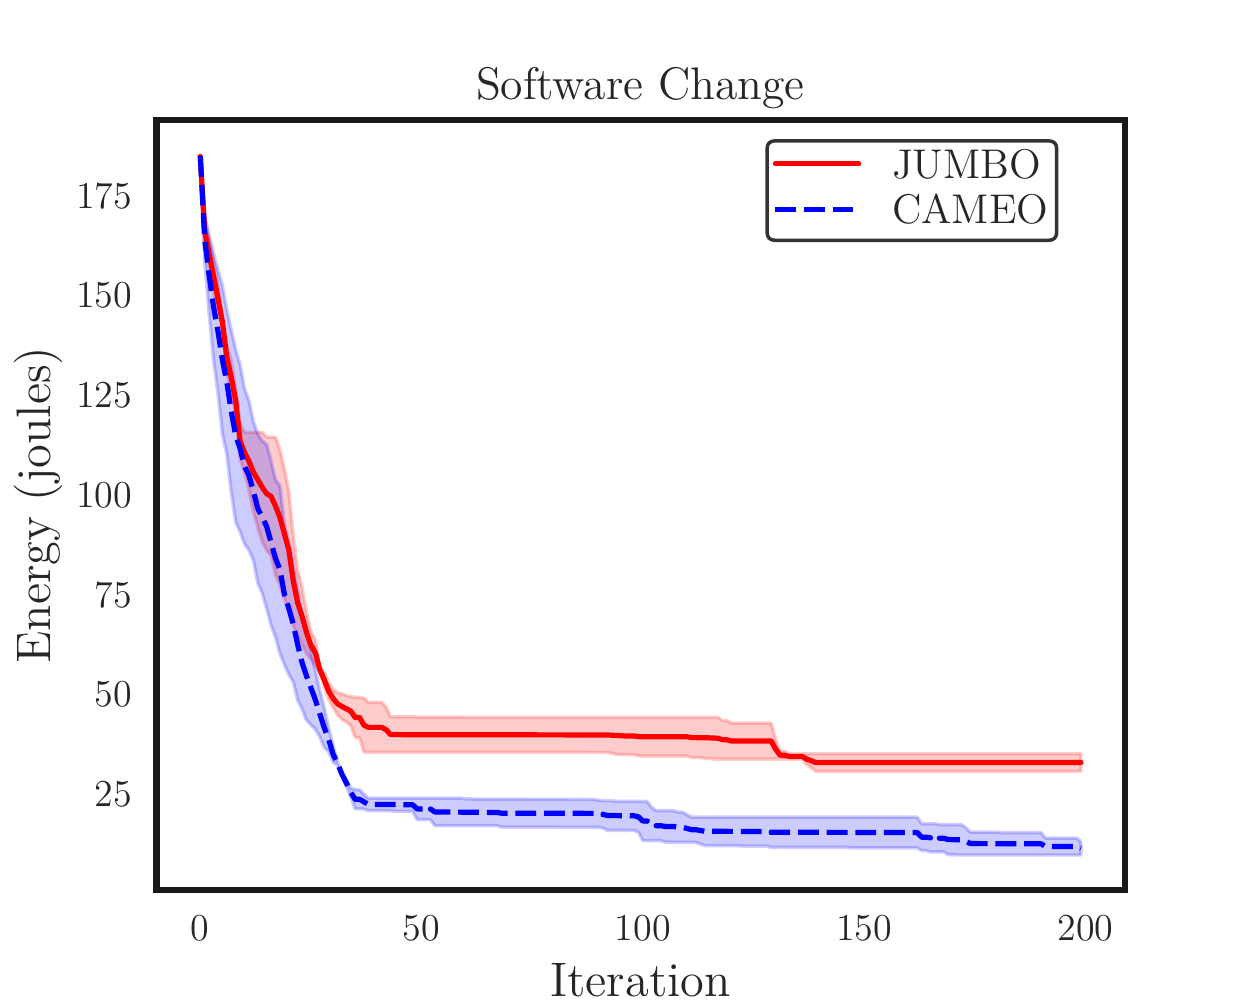}
  
%   \includegraphics[width=0.3\textwidth]{Figures/rq1_model_latency.pdf}
%   \includegraphics[width=0.3\textwidth]{Figures/rq1_workload_latency.pdf}
  \caption{\small{Effectiveness of \ourapproach when software changes in the deployment environment.}}
   \label{fig:rq1_app_software}
\vspace{-3mm}
\end{figure}

\begin{figure}[ht]
  \centering
  \includegraphics[width=0.48\columnwidth]{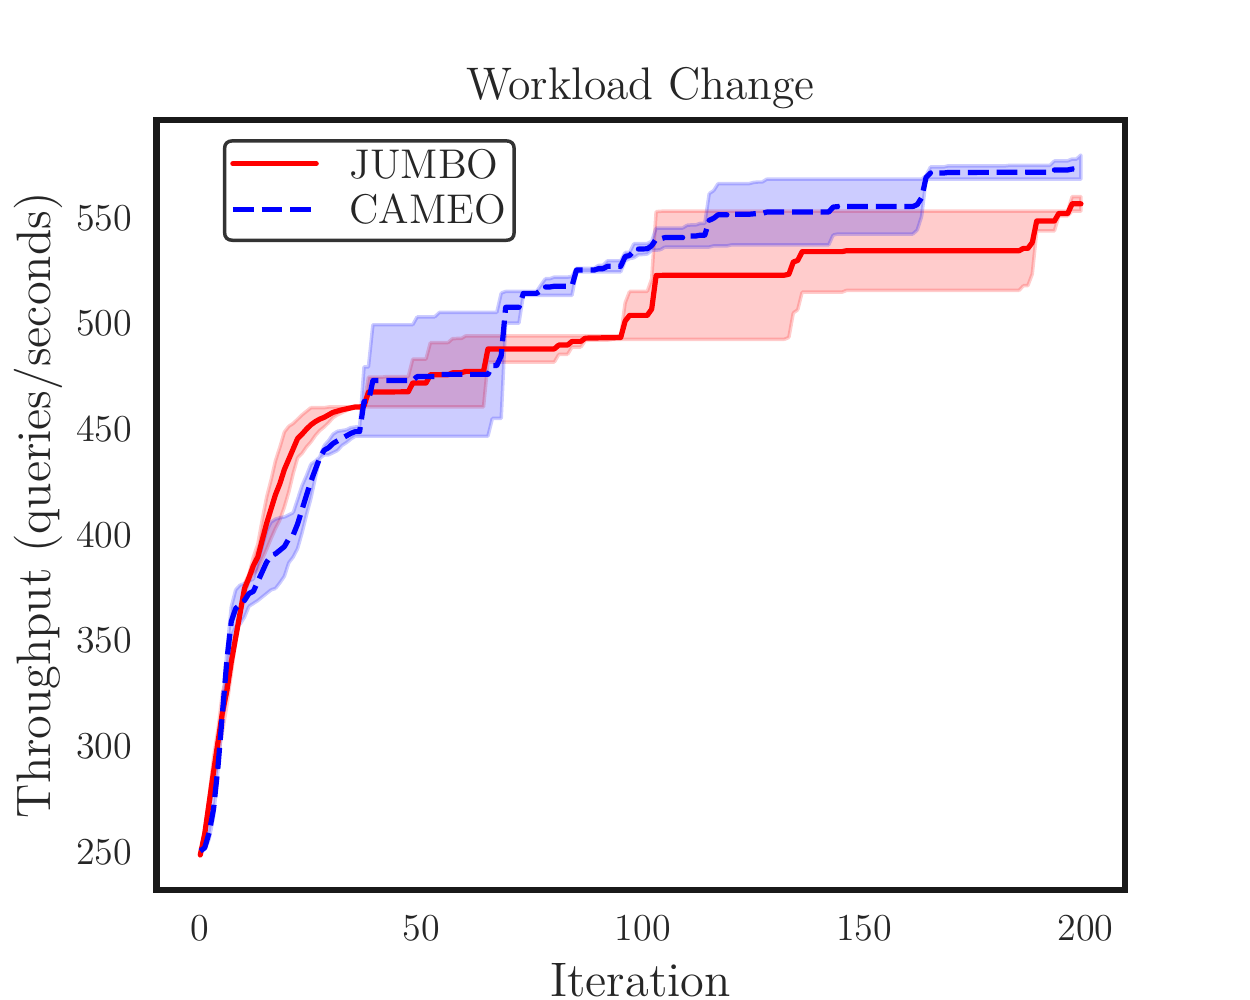}
  \includegraphics[width=0.48\columnwidth]{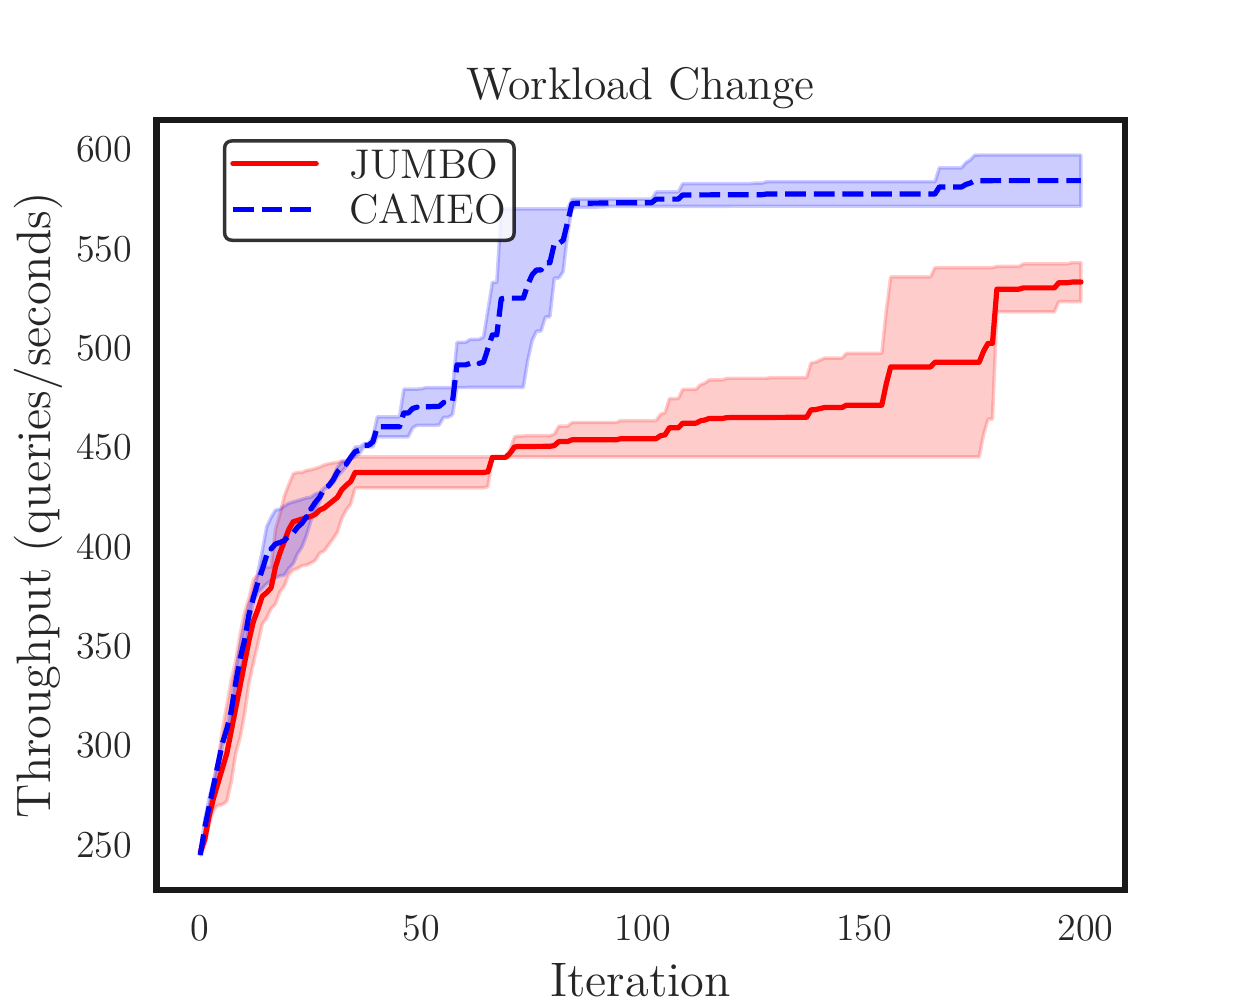}
  
%   \includegraphics[width=0.3\textwidth]{Figures/rq1_model_latency.pdf}
%   \includegraphics[width=0.3\textwidth]{Figures/rq1_workload_latency.pdf}
  \caption{\small{Effectiveness of \ourapproach when workload changes in the deployment environment.}}
   \label{fig:rq1_app_workload}
\vspace{-3mm}
\end{figure}

\begin{figure}[ht]
  \centering
  \includegraphics[width=0.48\columnwidth]{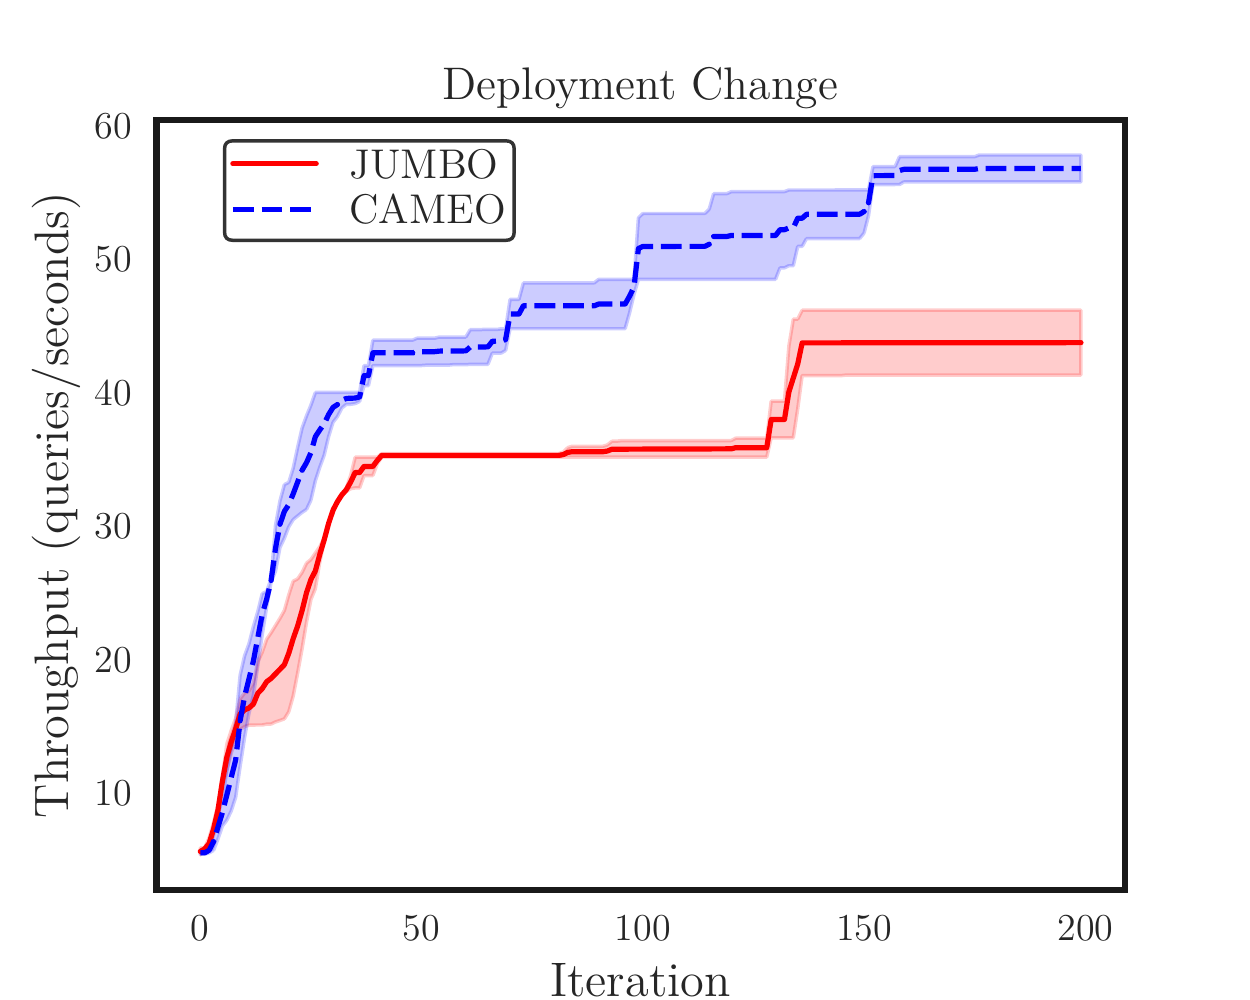}
  \includegraphics[width=0.48\columnwidth]{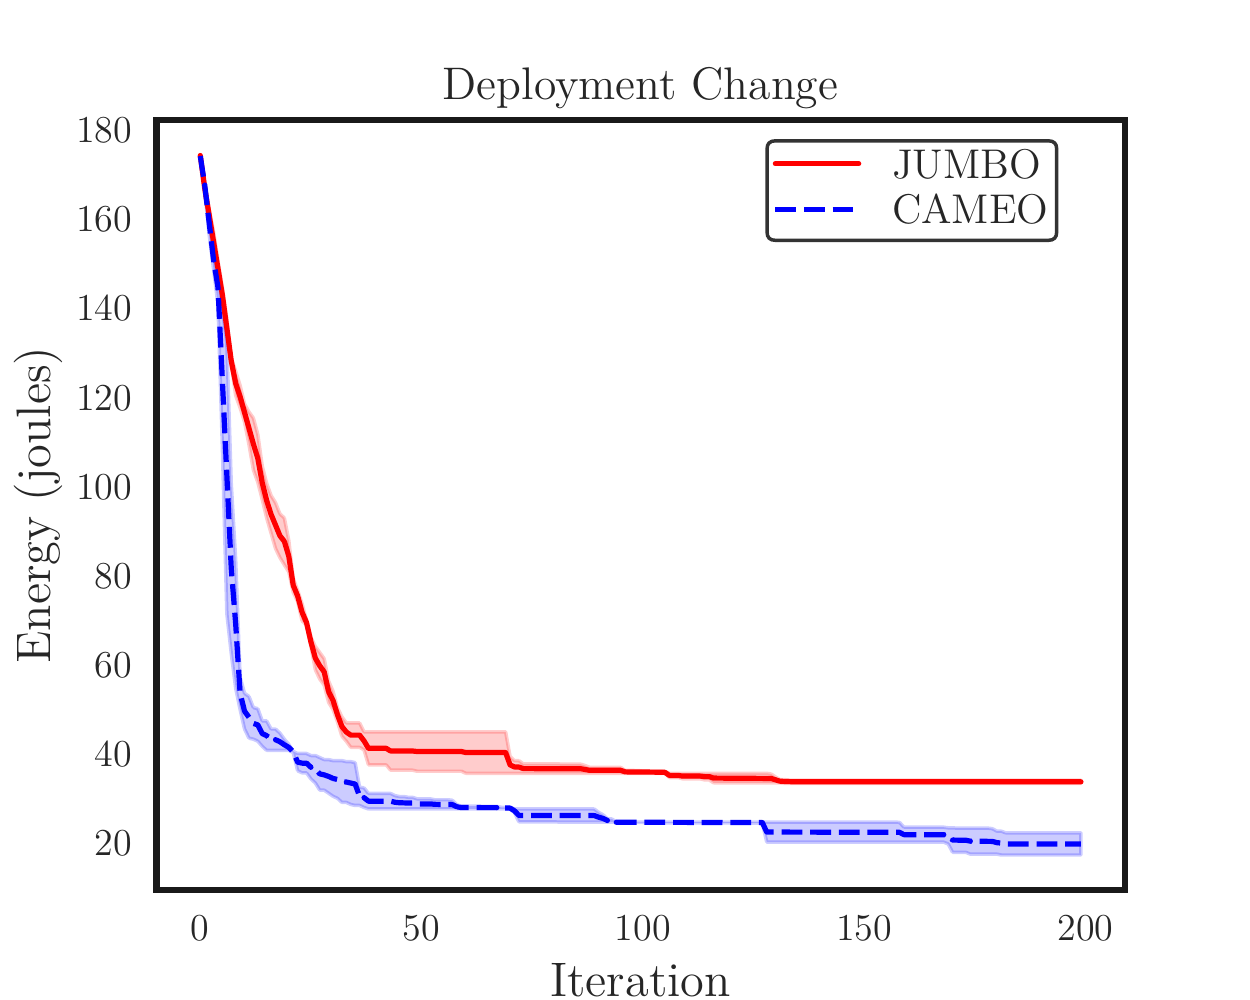}
  
%   \includegraphics[width=0.3\textwidth]{Figures/rq1_model_latency.pdf}
%   \includegraphics[width=0.3\textwidth]{Figures/rq1_workload_latency.pdf}
  \caption{\small{Effectiveness of \ourapproach when deployment topology changes in the deployment environment.}}
   \label{fig:rq1_app_deployment}
\vspace{-3mm}
\end{figure}

\subsection{RQ2 Additional Results}
% \begin{figure}[H]
%     \centering
%     \includegraphics[width=0.48\textwidth]{Figures/rq1_software_change.pdf}
%     \caption{Experimental setup when a software change takes place from {TinyBERT} to {BERT-Base} in the target for a NLP system.}
%     \label{fig:software_change_dep}
% \end{figure}
% \begin{figure}[ht]
\begin{figure}[H]
  \centering
  \includegraphics[width=0.32\linewidth]{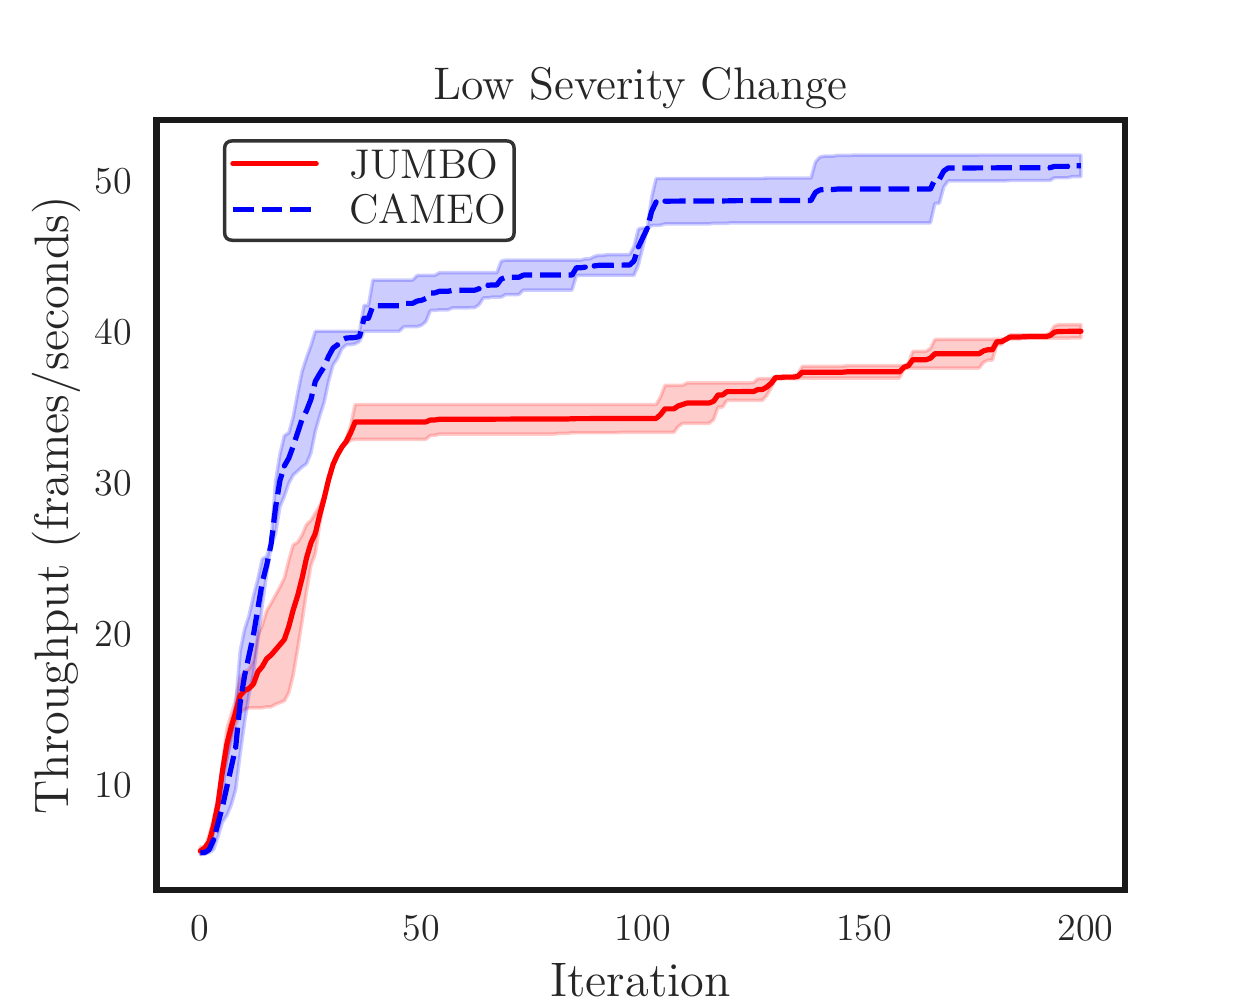}
  \includegraphics[width=0.32\linewidth]{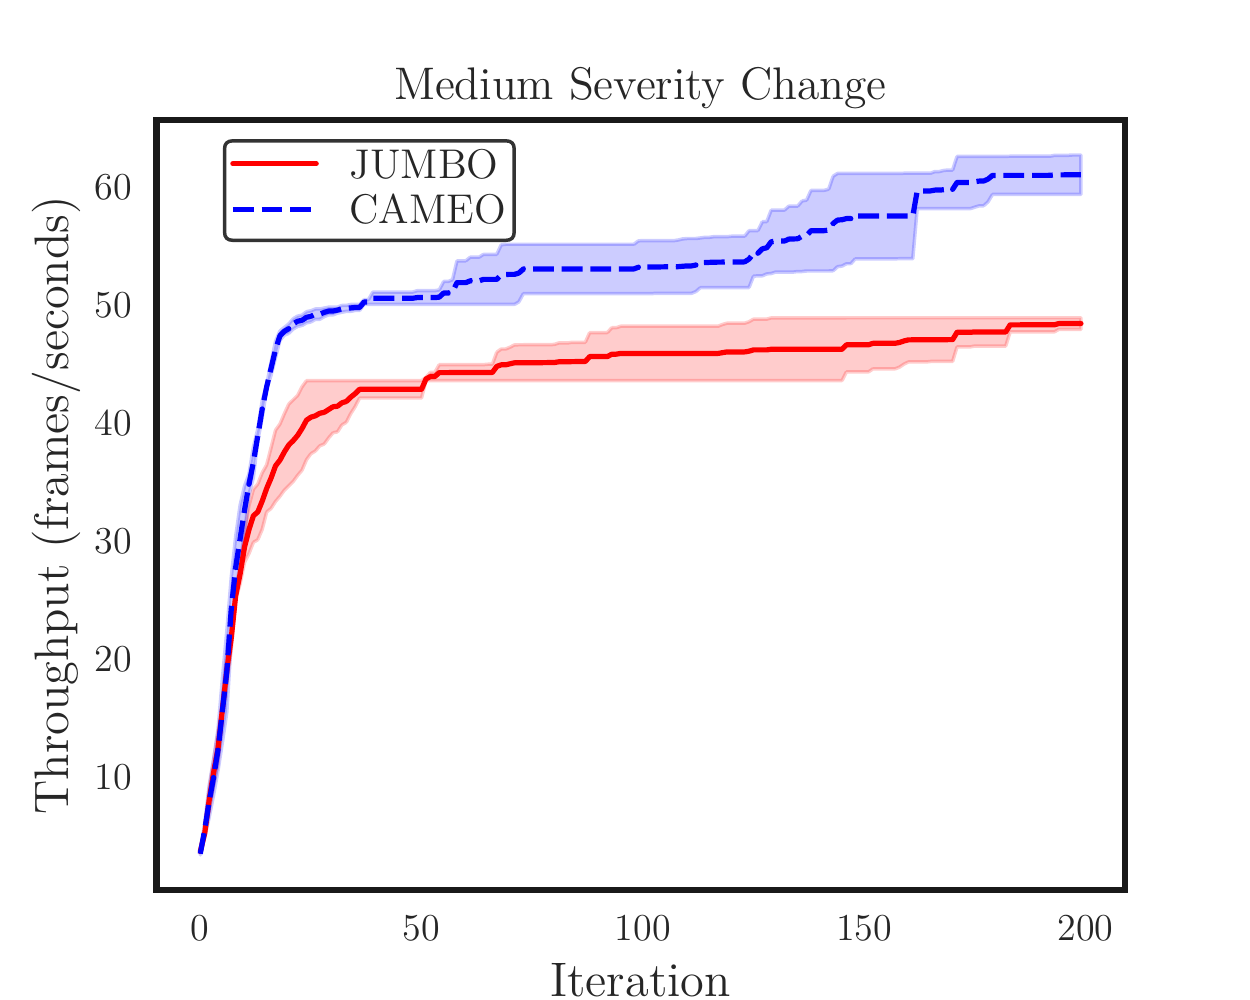}
   \includegraphics[width=0.32\linewidth]{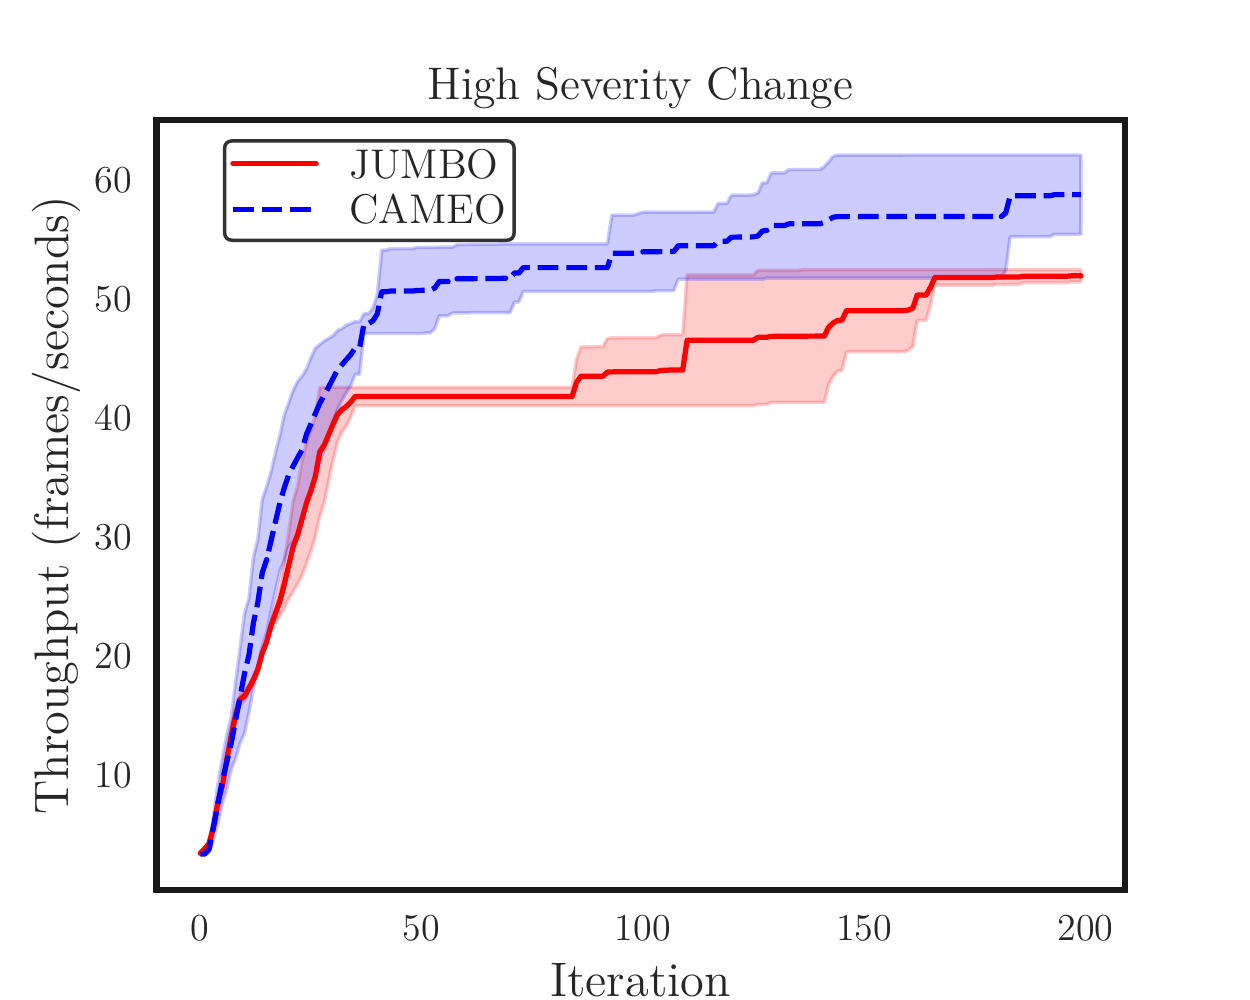}
%   \includegraphics[width=0.3\textwidth]{Figures/rq1_model_latency.pdf}
%   \includegraphics[width=0.3\textwidth]{Figures/rq1_workload_latency.pdf}
  \caption{\small{Effectiveness of \ourapproach when different severity of environmental changes happen in the deployment environment.}}
  \label{fig:rq2_app_severity}

\end{figure}
